# Supplementary material for: ReWiTe: Realistic Wide-angle and Telephoto Dual Camera Fusion Dataset via Beam Splitter Camera Rig
Source: arXiv:2404.10584 source file (2024-04-30)
Supplement: Supplementary file 1 [file sm.tex]

\section{Supplementary Materials}

First, we provide an overview of all images of our ReWiTe dataset in Figs.\ref{figure:dataset show} to \ref{figure:dataset show2}. 

Second, we provide more example results of the comparison algorithms, which are trained on the CameraFusion dataset vs. on our ReWiTe dataset in Figs. \ref{fig: result compare3} to \ref{fig: result compare11}.

\begin{figure*}
    \centering
    \includegraphics[width=.85\textwidth]{./figs/dataset_show.png}
    \vspace{-5pt}
    \caption{An overview of all images in ReWiTe. We only show the input {\bf{W}} images here for simplification.}
    \label{figure:dataset show}
\end{figure*}

\begin{figure*}
    \centering
    \includegraphics[width=.85\textwidth]{./figs/dataset_show2.png}
    \vspace{-5pt}
    \caption{An overview of all images in ReWiTe. We only show the input {\bf{W}} images here for simplification.}
    \label{figure:dataset show2}
\end{figure*}

\begin{figure*}
    \centering
    \begin{minipage}[b]{0.138\textwidth}
        \centering
        \setlength{\abovecaptionskip}{0.005cm}
       % \includegraphics[width=.98\textwidth]{./compare/dcsr/615.jpg}
       % \includegraphics[width=.98\textwidth]{./compare/dcsr/615_crop.jpg}
       % \includegraphics[width=.98\textwidth]{./compare/dcsr-fin/615_crop.jpg}
    %    \includegraphics[width=.98\textwidth]{./compare/gt/615_crop.jpg}
    %    \caption*{srntt}
       \includegraphics[width=.98\textwidth]{./compare/tele/40.jpg}
       \includegraphics[width=.98\textwidth]{./compare/tele/40_crop.jpg}
       \includegraphics[width=.98\textwidth]{./compare/tele/40_crop.jpg}
       % \includegraphics[width=.98\textwidth]{./compare/tele/40_crop.jpg}
    %    \includegraphics[width=.98\textwidth]{./compare/gt/40_crop.jpg}
        % \vspace{-6pt}
        \caption*{\bf{Input T}}
    \end{minipage}
    \begin{minipage}[b]{0.138\textwidth}
    \centering
        \setlength{\abovecaptionskip}{0.005cm}
       % \includegraphics[width=.98\textwidth]{./compare/dcsr/615.jpg}
       % \includegraphics[width=.98\textwidth]{./compare/dcsr/615_crop.jpg}
       % \includegraphics[width=.98\textwidth]{./compare/dcsr-fin/615_crop.jpg}
    %    \includegraphics[width=.98\textwidth]{./compare/gt/615_crop.jpg}
    %    \caption*{srntt}
       \includegraphics[width=.98\textwidth]{./compare/w+t/40.jpg}
       \includegraphics[width=.98\textwidth]{./compare/w+t/40_crop.jpg}
       \includegraphics[width=.98\textwidth]{./compare/w+t/40_crop.jpg}
       % \includegraphics[width=.98\textwidth]{./compare/tele/40_crop.jpg}
    %    \includegraphics[width=.98\textwidth]{./compare/gt/40_crop.jpg}
        % \vspace{-6pt}
        \caption*{\bf{Input W}}
    \end{minipage}
    \begin{minipage}[b]{0.138\textwidth}
        \centering
        \setlength{\abovecaptionskip}{0.005cm}
       % \includegraphics[width=.98\textwidth]{./compare/dcsr/615.jpg}
       % \includegraphics[width=.98\textwidth]{./compare/dcsr/615_crop.jpg}
       % \includegraphics[width=.98\textwidth]{./compare/dcsr-fin/615_crop.jpg}
    %    \includegraphics[width=.98\textwidth]{./compare/gt/615_crop.jpg}
    %    \caption*{srntt}
       \includegraphics[width=.98\textwidth]{./compare/c2/40.jpg}
       \includegraphics[width=.98\textwidth]{./compare/c2/40_crop.jpg}
       \includegraphics[width=.98\textwidth]{./compare/c2-fin/40_crop.jpg}
    %    \includegraphics[width=.98\textwidth]{./compare/gt/40_crop.jpg}
        % \vspace{-6pt}
        \caption*{C2-matching}
    \end{minipage}
    \begin{minipage}[b]{0.138\textwidth}
        \centering
        \setlength{\abovecaptionskip}{0.005cm}
       % \includegraphics[width=.98\textwidth]{./compare/dcsr/615.jpg}
       % \includegraphics[width=.98\textwidth]{./compare/dcsr/615_crop.jpg}
       % \includegraphics[width=.98\textwidth]{./compare/dcsr-fin/615_crop.jpg}
    %    \includegraphics[width=.98\textwidth]{./compare/gt/615_crop.jpg}
    %    \caption*{srntt}
       \includegraphics[width=.98\textwidth]{./compare/dcsr/40.jpg}
       \includegraphics[width=.98\textwidth]{./compare/dcsr/40_crop.jpg}
       \includegraphics[width=.98\textwidth]{./compare/dcsr-fin/40_crop.jpg}
    %    \includegraphics[width=.98\textwidth]{./compare/gt/40_crop.jpg}
        % \vspace{-6pt}
        \caption*{DCSR}
    \end{minipage}
    \begin{minipage}[b]{0.138\textwidth}
        \centering
        \setlength{\abovecaptionskip}{0.005cm}
       % \includegraphics[width=.98\textwidth]{./compare/selfdzsr/615.jpg}
       % \includegraphics[width=.98\textwidth]{./compare/selfdzsr/615_crop.jpg}
       % \includegraphics[width=.98\textwidth]{./compare/selfdzsr-fin/615_crop.jpg}
    %    \includegraphics[width=.98\textwidth]{./compare/gt/615_crop.jpg}
    %    \caption*{srntt}
       \includegraphics[width=.98\textwidth]{./compare/selfdzsr/40.jpg}
       \includegraphics[width=.98\textwidth]{./compare/selfdzsr/40_crop.jpg}
       \includegraphics[width=.98\textwidth]{./compare/selfdzsr-fin/40_crop.jpg}
    %    \includegraphics[width=.98\textwidth]{./compare/gt/40_crop.jpg}
        % \vspace{-6pt}
        \caption*{SelfDZSR}
    \end{minipage}
    \begin{minipage}[b]{0.138\textwidth}
        \centering
        \setlength{\abovecaptionskip}{0.005cm}
       % \includegraphics[width=.98\textwidth]{./compare/zedusr/615.jpg}
       % \includegraphics[width=.98\textwidth]{./compare/zedusr/615_crop.jpg}
       % \includegraphics[width=.98\textwidth]{./compare/zedusr-fin/615_crop.jpg}
    %    \includegraphics[width=.98\textwidth]{./compare/gt/615_crop.jpg}
    %    \caption*{srntt}
       \includegraphics[width=.98\textwidth]{./compare/zedusr/40.jpg}
       \includegraphics[width=.98\textwidth]{./compare/zedusr/40_crop.jpg}
       \includegraphics[width=.98\textwidth]{./compare/zedusr-fin/40_crop.jpg}
    %    \includegraphics[width=.98\textwidth]{./compare/gt/40_crop.jpg}
        % \vspace{-6pt}
        \caption*{ZeDUSR}
    \end{minipage}
    \begin{minipage}[b]{0.138\textwidth}
        \centering
        \setlength{\abovecaptionskip}{0.005cm}
       % \includegraphics[width=.98\textwidth]{./compare/MASA/615.jpg}
       % \includegraphics[width=.98\textwidth]{./compare/MASA/615_crop.jpg}
       % \includegraphics[width=.98\textwidth]{./compare/MASA-fin/615_crop.jpg}
    %    \includegraphics[width=.98\textwidth]{./compare/gt/615_crop.jpg}
    %    \caption*{srntt}
       \includegraphics[width=.98\textwidth]{./compare/MASA/40.jpg}
       \includegraphics[width=.98\textwidth]{./compare/MASA/40_crop.jpg}
       \includegraphics[width=.98\textwidth]{./compare/MASA-fin/40_crop.jpg}
    %    \includegraphics[width=.98\textwidth]{./compare/gt/40_crop.jpg}
        % \vspace{-6pt}
        \caption*{MASA}
    \end{minipage}
    \begin{minipage}[b]{0.138\textwidth}
        \centering
        \setlength{\abovecaptionskip}{0.005cm}
       % \includegraphics[width=.98\textwidth]{./compare/ttsr/615.jpg}
       % \includegraphics[width=.98\textwidth]{./compare/ttsr/615_crop.jpg}
       % \includegraphics[width=.98\textwidth]{./compare/ttsr-fin/615_crop.jpg}
    %    \includegraphics[width=.98\textwidth]{./compare/gt/615_crop.jpg}
    %    \caption*{srntt}
       \includegraphics[width=.98\textwidth]{./compare/ttsr/40.jpg}
       \includegraphics[width=.98\textwidth]{./compare/ttsr/40_crop.jpg}
       \includegraphics[width=.98\textwidth]{./compare/ttsr-fin/40_crop.jpg}
    %    \includegraphics[width=.98\textwidth]{./compare/gt/40_crop.jpg}
        % \vspace{-6pt}
        \caption*{TTSR}
    \end{minipage}
    \begin{minipage}[b]{0.138\textwidth}
        \centering
        \setlength{\abovecaptionskip}{0.005cm}
       % \includegraphics[width=.98\textwidth]{./compare/srntt/615.jpg}
       % \includegraphics[width=.98\textwidth]{./compare/srntt/615_crop.jpg}
       % \includegraphics[width=.98\textwidth]{./compare/srntt-fin/615_crop.jpg}
    %    \includegraphics[width=.98\textwidth]{./compare/gt/615_crop.jpg}
    %    \caption*{srntt}
       \includegraphics[width=.98\textwidth]{./compare/srntt/40.jpg}
       \includegraphics[width=.98\textwidth]{./compare/srntt/40_crop.jpg}
       \includegraphics[width=.98\textwidth]{./compare/srntt-fin/40_crop.jpg}
    %    \includegraphics[width=.98\textwidth]{./compare/gt/40_crop.jpg}
        % \vspace{-6pt}
        \caption*{SRNTT}
    \end{minipage}
    \begin{minipage}[b]{0.138\textwidth}
        \centering
        \setlength{\abovecaptionskip}{0.005cm}
       % \includegraphics[width=.98\textwidth]{./compare/RCAN/615.jpg}
       % \includegraphics[width=.98\textwidth]{./compare/RCAN/615_crop.jpg}
       % \includegraphics[width=.98\textwidth]{./compare/RCAN-fin/615_crop.jpg}
    %    \includegraphics[width=.98\textwidth]{./compare/gt/615_crop.jpg}
    %    \caption*{RCAN}
       \includegraphics[width=.98\textwidth]{./compare/RCAN/40.jpg}
       \includegraphics[width=.98\textwidth]{./compare/RCAN/40_crop.jpg}
       \includegraphics[width=.98\textwidth]{./compare/RCAN-fin/40_crop.jpg}
    %    \includegraphics[width=.98\textwidth]{./compare/gt/40_crop.jpg}
        % \vspace{-6pt}
        \caption*{RCAN}
    \end{minipage}
    \begin{minipage}[b]{0.138\textwidth}
        \centering
        \setlength{\abovecaptionskip}{0.005cm}
       % \includegraphics[width=.98\textwidth]{./compare/EDSR/615.jpg}
       % \includegraphics[width=.98\textwidth]{./compare/EDSR/615_crop.jpg}
       % \includegraphics[width=.98\textwidth]{./compare/EDSR-fin/615_crop.jpg}
    %    \includegraphics[width=.98\textwidth]{./compare/gt/615_crop.jpg}
    %    \caption*{EDSR}
       \includegraphics[width=.98\textwidth]{./compare/EDSR/40.jpg}
       \includegraphics[width=.98\textwidth]{./compare/EDSR/40_crop.jpg}
       \includegraphics[width=.98\textwidth]{./compare/EDSR-fin/40_crop.jpg}
    %    \includegraphics[width=.98\textwidth]{./compare/gt/40_crop.jpg}
        % \vspace{-6pt}
        \caption*{EDSR}
    \end{minipage}
    \begin{minipage}[b]{0.138\textwidth}
        \centering
        \setlength{\abovecaptionskip}{0.005cm}
       % \includegraphics[width=.98\textwidth]{./compare/Real_ESRGAN/615.jpg}
       % \includegraphics[width=.98\textwidth]{./compare/Real_ESRGAN/615_crop.jpg}
       % \includegraphics[width=.98\textwidth]{./compare/Real_ESRGAN-fin/615_crop.jpg}
    %    \includegraphics[width=.98\textwidth]{./compare/gt/615_crop.jpg}
    %    \caption*{Real_ESRGAN}
       \includegraphics[width=.98\textwidth]{./compare/Real_ESRGAN/40.jpg}
       \includegraphics[width=.98\textwidth]{./compare/Real_ESRGAN/40_crop.jpg}
       \includegraphics[width=.98\textwidth]{./compare/Real_ESRGAN-fin/40_crop.jpg}
    %    \includegraphics[width=.98\textwidth]{./compare/gt/40_crop.jpg}
        % \vspace{-6pt}
        \caption*{Real-ESRGAN}
    \end{minipage}
    \begin{minipage}[b]{0.138\textwidth}
        \centering
        \setlength{\abovecaptionskip}{0.005cm}
       % \includegraphics[width=.98\textwidth]{./compare/swinir/615.jpg}
       % \includegraphics[width=.98\textwidth]{./compare/swinir/615_crop.jpg}
       % \includegraphics[width=.98\textwidth]{./compare/swinir-fin/615_crop.jpg}
    %    \includegraphics[width=.98\textwidth]{./compare/gt/615_crop.jpg}
    %    \caption*{SwinIR}
       \includegraphics[width=.98\textwidth]{./compare/swinir/40.jpg}
       \includegraphics[width=.98\textwidth]{./compare/swinir/40_crop.jpg}
       \includegraphics[width=.98\textwidth]{./compare/swinir-fin/40_crop.jpg}
    %    \includegraphics[width=.98\textwidth]{./compare/gt/40_crop.jpg}
        % \vspace{-6pt}
        \caption*{SwinIR}
    \end{minipage}
    \begin{minipage}[b]{0.138\textwidth}
        \centering
        \setlength{\abovecaptionskip}{0.005cm}
       % \includegraphics[width=.98\textwidth]{./compare/gt/615.jpg}
    %    \includegraphics[width=.98\textwidth]{./compare/swinir/615_crop.jpg}
    %    \includegraphics[width=.98\textwidth]{./compare/swinir-fin/615_crop.jpg}
       % \includegraphics[width=.98\textwidth]{./compare/gt/615_crop.jpg}
    %    \caption*{SwinIR}
       \includegraphics[width=.98\textwidth]{./compare/gt/40.jpg}
       \includegraphics[width=.98\textwidth]{./compare/gt/40_crop.jpg}
       \includegraphics[width=.98\textwidth]{./compare/gt/40_crop.jpg}
        % \vspace{-6pt}
        \caption*{GT}
    \end{minipage}
    \vspace{-10pt}
    \caption{Example results of different algorithms trained on CameraFusion vs. ReWiTe. Top: The full-image results of different algorithms trained on ReWiTe. Middle: Results focused on the red-box region, derived from algorithms trained on CameraFusion. Bottom: Results focused on the red-box region, derived from algorithms trained on ReWiTe. Since the difficulty of perceiving differences of full-image results in compressed image size, only one full-image result is shown in the top line.
    }
    \label{fig: result compare3}
\end{figure*}

\begin{figure*}
    \centering
    \begin{minipage}[b]{0.138\textwidth}
        \centering
        \setlength{\abovecaptionskip}{0.005cm}
       % \includegraphics[width=.98\textwidth]{./compare/dcsr/615.jpg}
       % \includegraphics[width=.98\textwidth]{./compare/dcsr/615_crop.jpg}
       % \includegraphics[width=.98\textwidth]{./compare/dcsr-fin/615_crop.jpg}
    %    \includegraphics[width=.98\textwidth]{./compare/gt/615_crop.jpg}
    %    \caption*{srntt}
       \includegraphics[width=.98\textwidth]{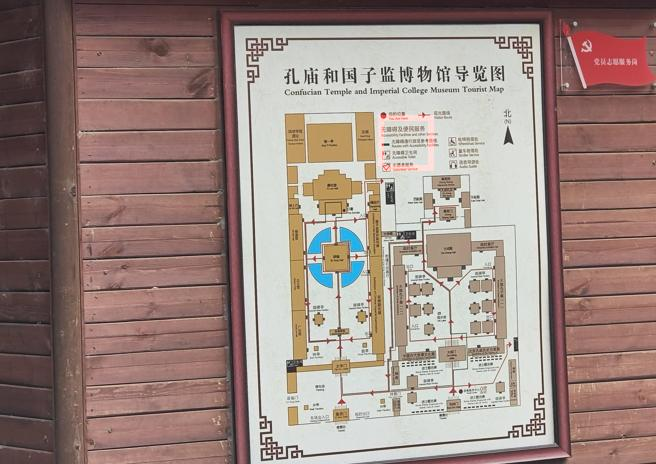}
       \includegraphics[width=.98\textwidth]{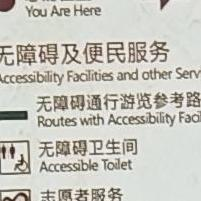}
       \includegraphics[width=.98\textwidth]{./compare/tele/336_crop.jpg}
       % \includegraphics[width=.98\textwidth]{./compare/tele/336_crop.jpg}
    %    \includegraphics[width=.98\textwidth]{./compare/gt/336_crop.jpg}
        % \vspace{-6pt}
        \caption*{\bf{Input T}}
    \end{minipage}
    \begin{minipage}[b]{0.138\textwidth}
    \centering
        \setlength{\abovecaptionskip}{0.005cm}
       % \includegraphics[width=.98\textwidth]{./compare/dcsr/615.jpg}
       % \includegraphics[width=.98\textwidth]{./compare/dcsr/615_crop.jpg}
       % \includegraphics[width=.98\textwidth]{./compare/dcsr-fin/615_crop.jpg}
    %    \includegraphics[width=.98\textwidth]{./compare/gt/615_crop.jpg}
    %    \caption*{srntt}
       \includegraphics[width=.98\textwidth]{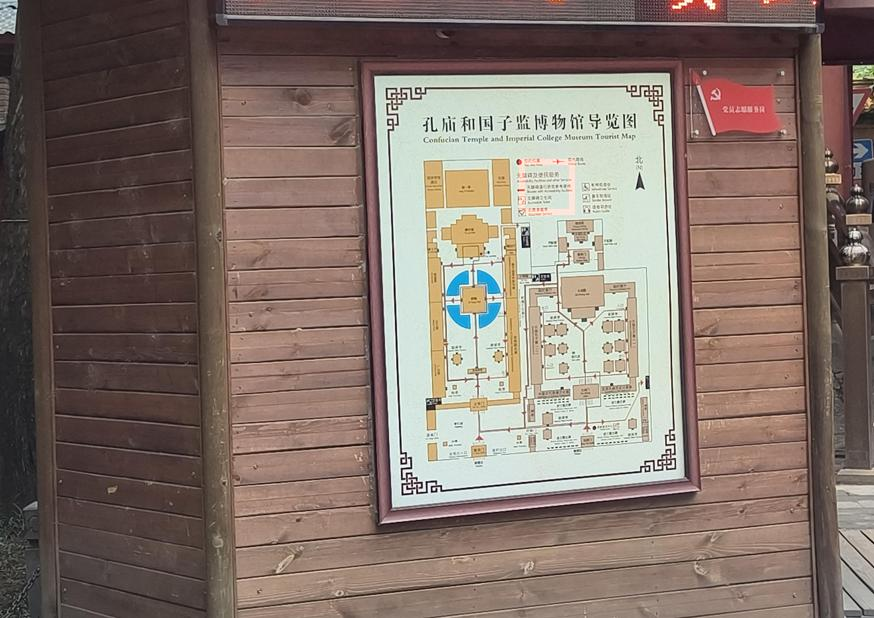}
       \includegraphics[width=.98\textwidth]{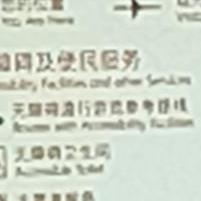}
       \includegraphics[width=.98\textwidth]{./compare/w+t/336_crop.jpg}
       % \includegraphics[width=.98\textwidth]{./compare/tele/336_crop.jpg}
    %    \includegraphics[width=.98\textwidth]{./compare/gt/336_crop.jpg}
        % \vspace{-6pt}
        \caption*{\bf{Input W}}
    \end{minipage}
    \begin{minipage}[b]{0.138\textwidth}
        \centering
        \setlength{\abovecaptionskip}{0.005cm}
       % \includegraphics[width=.98\textwidth]{./compare/dcsr/615.jpg}
       % \includegraphics[width=.98\textwidth]{./compare/dcsr/615_crop.jpg}
       % \includegraphics[width=.98\textwidth]{./compare/dcsr-fin/615_crop.jpg}
    %    \includegraphics[width=.98\textwidth]{./compare/gt/615_crop.jpg}
    %    \caption*{srntt}
       \includegraphics[width=.98\textwidth]{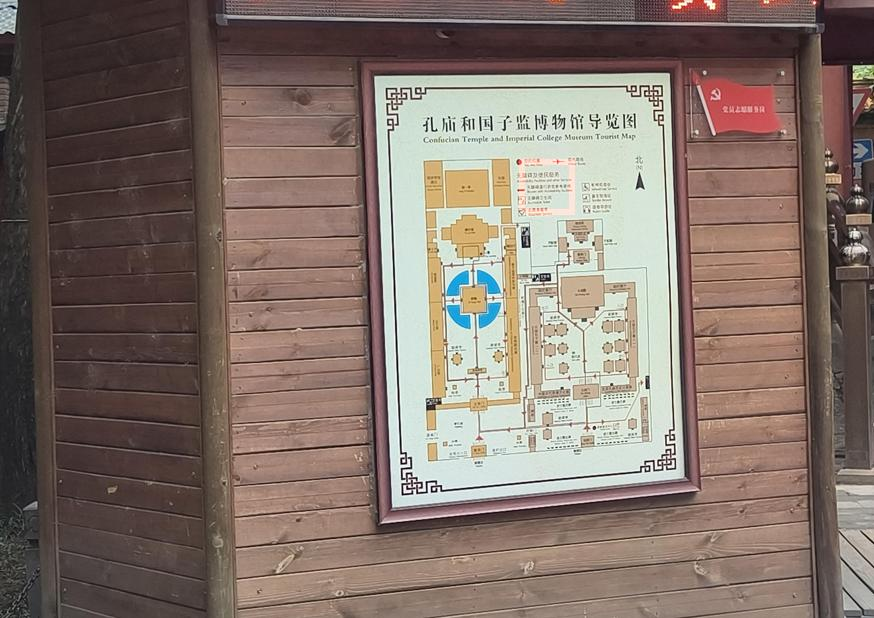}
       \includegraphics[width=.98\textwidth]{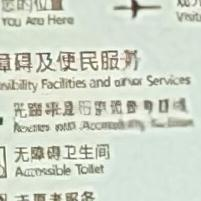}
       \includegraphics[width=.98\textwidth]{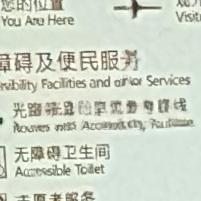}
    %    \includegraphics[width=.98\textwidth]{./compare/gt/336_crop.jpg}
        % \vspace{-6pt}
        \caption*{C2-matching}
    \end{minipage}
    \begin{minipage}[b]{0.138\textwidth}
        \centering
        \setlength{\abovecaptionskip}{0.005cm}
       % \includegraphics[width=.98\textwidth]{./compare/dcsr/615.jpg}
       % \includegraphics[width=.98\textwidth]{./compare/dcsr/615_crop.jpg}
       % \includegraphics[width=.98\textwidth]{./compare/dcsr-fin/615_crop.jpg}
    %    \includegraphics[width=.98\textwidth]{./compare/gt/615_crop.jpg}
    %    \caption*{srntt}
       \includegraphics[width=.98\textwidth]{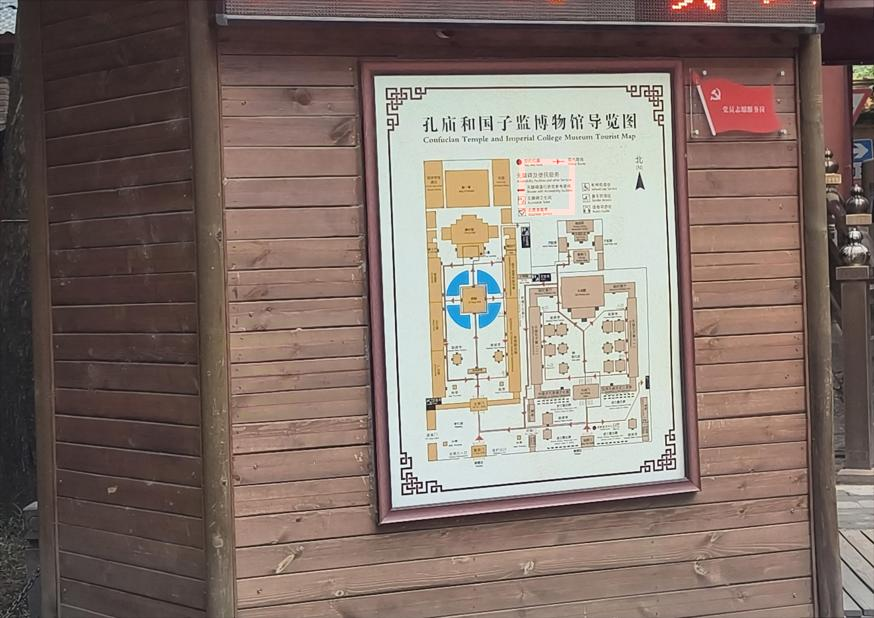}
       \includegraphics[width=.98\textwidth]{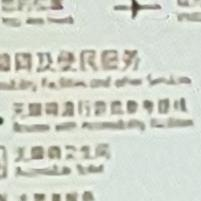}
       \includegraphics[width=.98\textwidth]{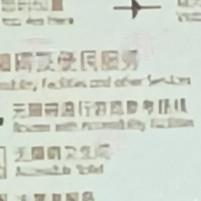}
    %    \includegraphics[width=.98\textwidth]{./compare/gt/336_crop.jpg}
        % \vspace{-6pt}
        \caption*{DCSR}
    \end{minipage}
    \begin{minipage}[b]{0.138\textwidth}
        \centering
        \setlength{\abovecaptionskip}{0.005cm}
       % \includegraphics[width=.98\textwidth]{./compare/selfdzsr/615.jpg}
       % \includegraphics[width=.98\textwidth]{./compare/selfdzsr/615_crop.jpg}
       % \includegraphics[width=.98\textwidth]{./compare/selfdzsr-fin/615_crop.jpg}
    %    \includegraphics[width=.98\textwidth]{./compare/gt/615_crop.jpg}
    %    \caption*{srntt}
       \includegraphics[width=.98\textwidth]{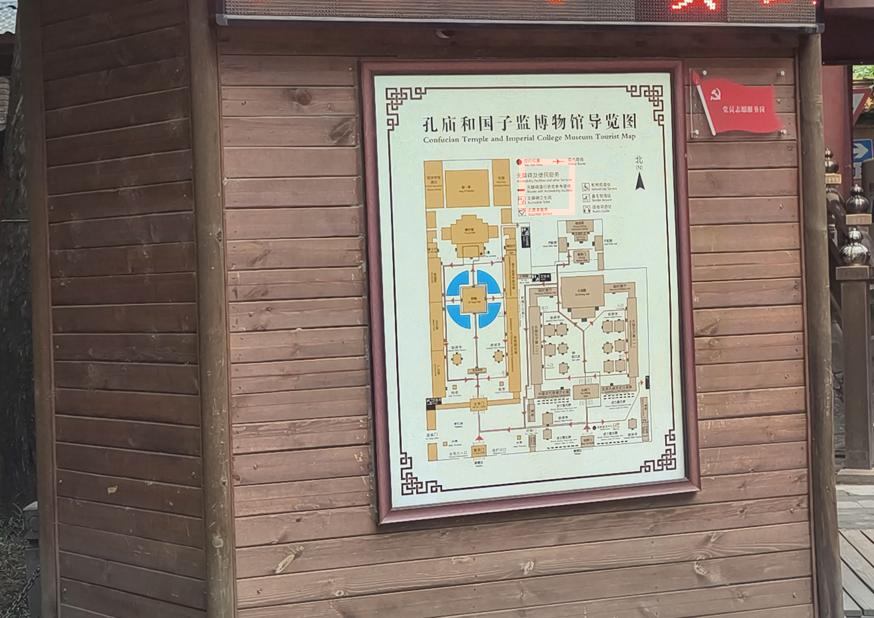}
       \includegraphics[width=.98\textwidth]{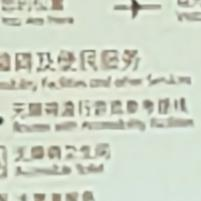}
       \includegraphics[width=.98\textwidth]{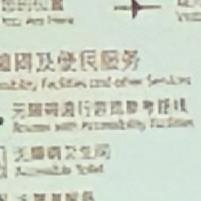}
    %    \includegraphics[width=.98\textwidth]{./compare/gt/336_crop.jpg}
        % \vspace{-6pt}
        \caption*{SelfDZSR}
    \end{minipage}
    \begin{minipage}[b]{0.138\textwidth}
        \centering
        \setlength{\abovecaptionskip}{0.005cm}
       % \includegraphics[width=.98\textwidth]{./compare/zedusr/615.jpg}
       % \includegraphics[width=.98\textwidth]{./compare/zedusr/615_crop.jpg}
       % \includegraphics[width=.98\textwidth]{./compare/zedusr-fin/615_crop.jpg}
    %    \includegraphics[width=.98\textwidth]{./compare/gt/615_crop.jpg}
    %    \caption*{srntt}
       \includegraphics[width=.98\textwidth]{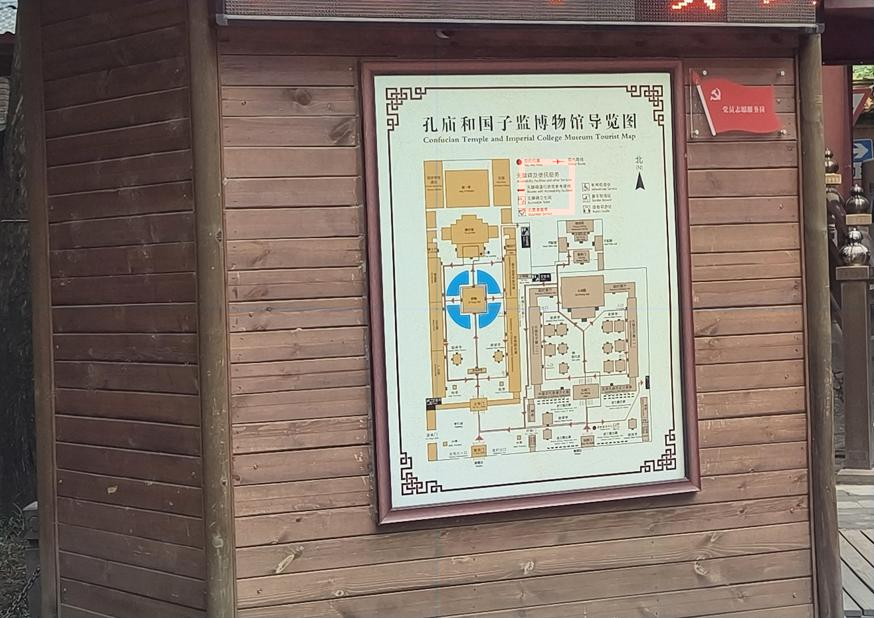}
       \includegraphics[width=.98\textwidth]{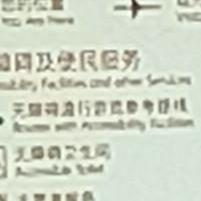}
       \includegraphics[width=.98\textwidth]{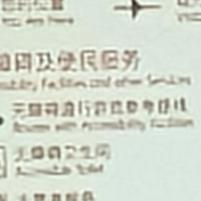}
    %    \includegraphics[width=.98\textwidth]{./compare/gt/336_crop.jpg}
        % \vspace{-6pt}
        \caption*{ZeDUSR}
    \end{minipage}
    \begin{minipage}[b]{0.138\textwidth}
        \centering
        \setlength{\abovecaptionskip}{0.005cm}
       % \includegraphics[width=.98\textwidth]{./compare/MASA/615.jpg}
       % \includegraphics[width=.98\textwidth]{./compare/MASA/615_crop.jpg}
       % \includegraphics[width=.98\textwidth]{./compare/MASA-fin/615_crop.jpg}
    %    \includegraphics[width=.98\textwidth]{./compare/gt/615_crop.jpg}
    %    \caption*{srntt}
       \includegraphics[width=.98\textwidth]{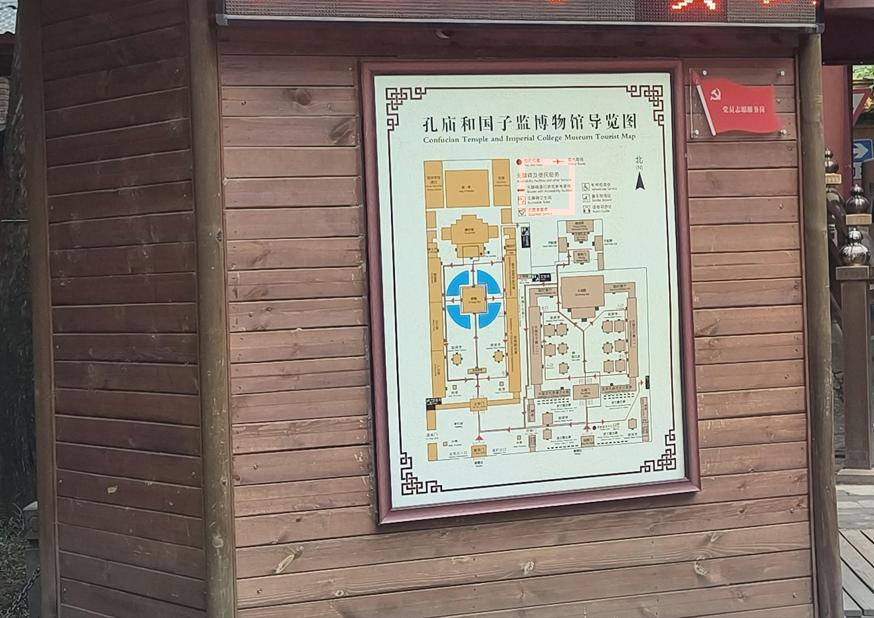}
       \includegraphics[width=.98\textwidth]{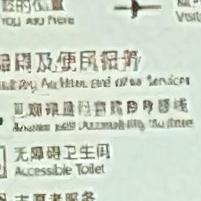}
       \includegraphics[width=.98\textwidth]{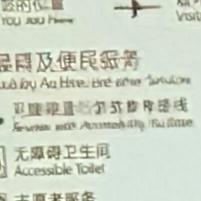}
    %    \includegraphics[width=.98\textwidth]{./compare/gt/336_crop.jpg}
        % \vspace{-6pt}
        \caption*{MASA}
    \end{minipage}
    \begin{minipage}[b]{0.138\textwidth}
        \centering
        \setlength{\abovecaptionskip}{0.005cm}
       % \includegraphics[width=.98\textwidth]{./compare/ttsr/615.jpg}
       % \includegraphics[width=.98\textwidth]{./compare/ttsr/615_crop.jpg}
       % \includegraphics[width=.98\textwidth]{./compare/ttsr-fin/615_crop.jpg}
    %    \includegraphics[width=.98\textwidth]{./compare/gt/615_crop.jpg}
    %    \caption*{srntt}
       \includegraphics[width=.98\textwidth]{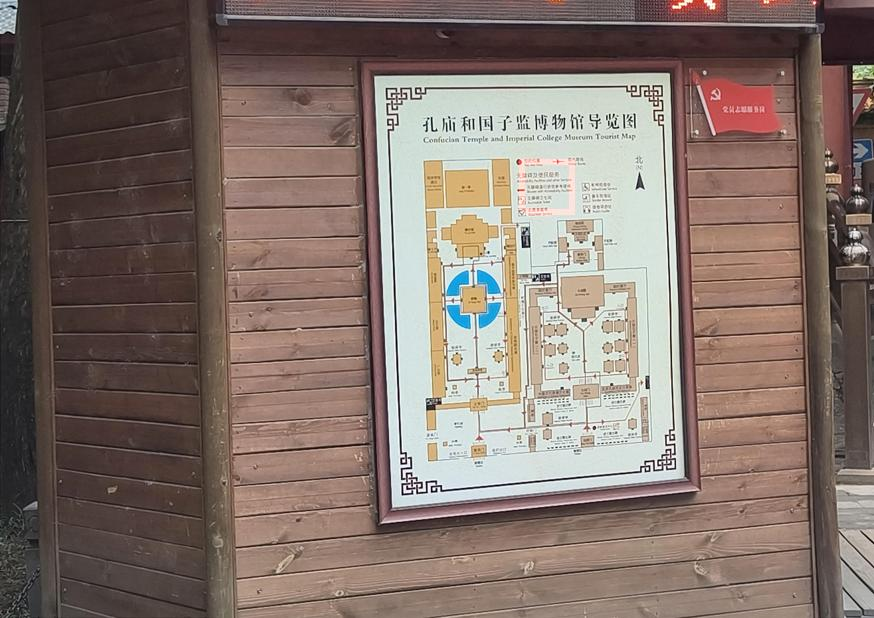}
       \includegraphics[width=.98\textwidth]{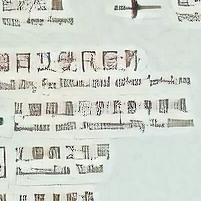}
       \includegraphics[width=.98\textwidth]{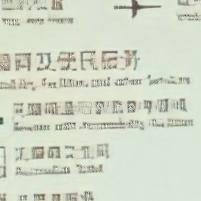}
    %    \includegraphics[width=.98\textwidth]{./compare/gt/336_crop.jpg}
        % \vspace{-6pt}
        \caption*{TTSR}
    \end{minipage}
    \begin{minipage}[b]{0.138\textwidth}
        \centering
        \setlength{\abovecaptionskip}{0.005cm}
       % \includegraphics[width=.98\textwidth]{./compare/srntt/615.jpg}
       % \includegraphics[width=.98\textwidth]{./compare/srntt/615_crop.jpg}
       % \includegraphics[width=.98\textwidth]{./compare/srntt-fin/615_crop.jpg}
    %    \includegraphics[width=.98\textwidth]{./compare/gt/615_crop.jpg}
    %    \caption*{srntt}
       \includegraphics[width=.98\textwidth]{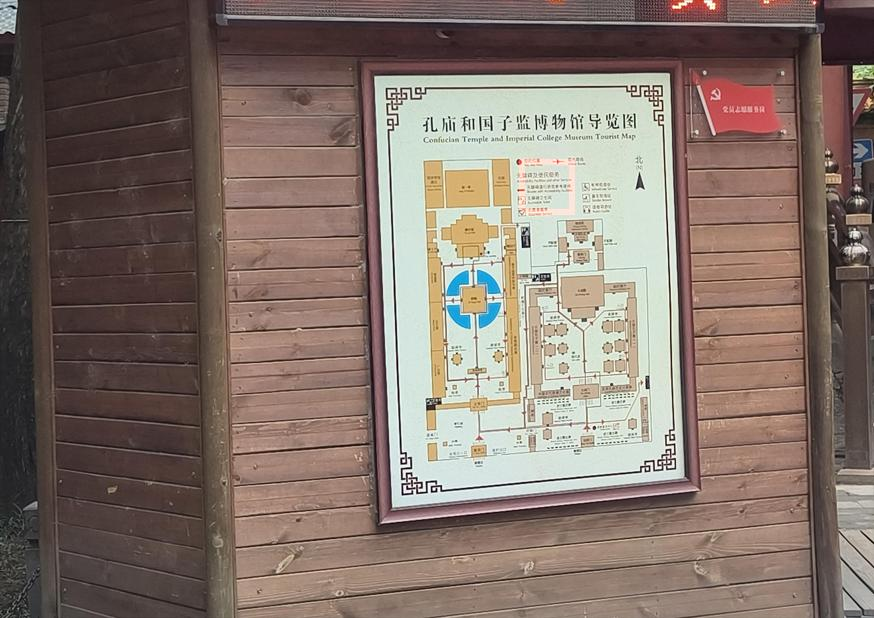}
       \includegraphics[width=.98\textwidth]{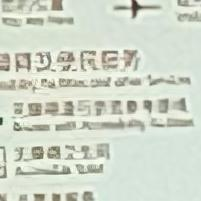}
       \includegraphics[width=.98\textwidth]{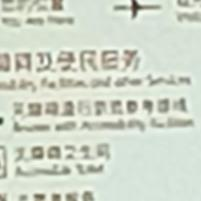}
    %    \includegraphics[width=.98\textwidth]{./compare/gt/336_crop.jpg}
        % \vspace{-6pt}
        \caption*{SRNTT}
    \end{minipage}
    \begin{minipage}[b]{0.138\textwidth}
        \centering
        \setlength{\abovecaptionskip}{0.005cm}
       % \includegraphics[width=.98\textwidth]{./compare/RCAN/615.jpg}
       % \includegraphics[width=.98\textwidth]{./compare/RCAN/615_crop.jpg}
       % \includegraphics[width=.98\textwidth]{./compare/RCAN-fin/615_crop.jpg}
    %    \includegraphics[width=.98\textwidth]{./compare/gt/615_crop.jpg}
    %    \caption*{RCAN}
       \includegraphics[width=.98\textwidth]{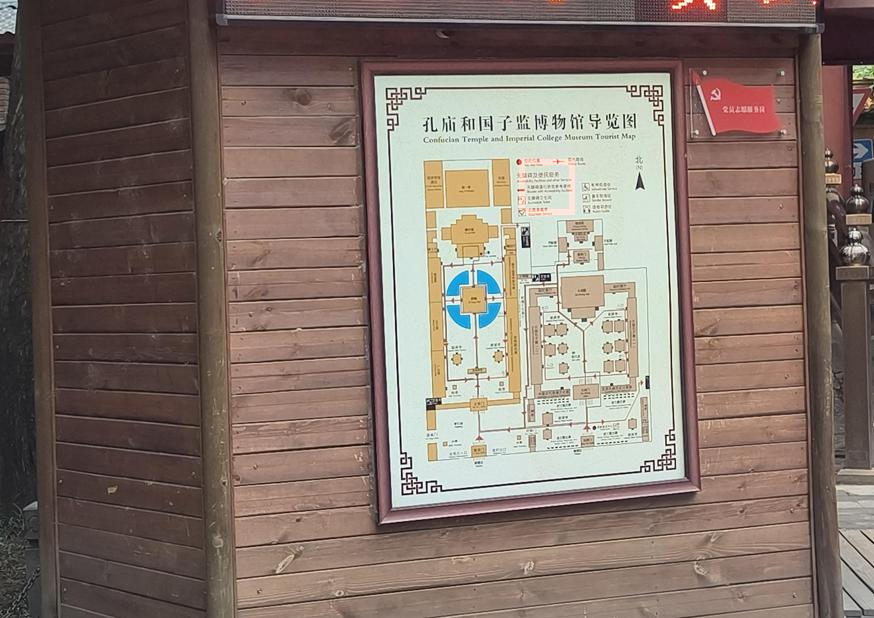}
       \includegraphics[width=.98\textwidth]{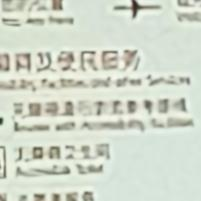}
       \includegraphics[width=.98\textwidth]{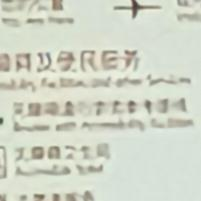}
    %    \includegraphics[width=.98\textwidth]{./compare/gt/336_crop.jpg}
        % \vspace{-6pt}
        \caption*{RCAN}
    \end{minipage}
    \begin{minipage}[b]{0.138\textwidth}
        \centering
        \setlength{\abovecaptionskip}{0.005cm}
       % \includegraphics[width=.98\textwidth]{./compare/EDSR/615.jpg}
       % \includegraphics[width=.98\textwidth]{./compare/EDSR/615_crop.jpg}
       % \includegraphics[width=.98\textwidth]{./compare/EDSR-fin/615_crop.jpg}
    %    \includegraphics[width=.98\textwidth]{./compare/gt/615_crop.jpg}
    %    \caption*{EDSR}
       \includegraphics[width=.98\textwidth]{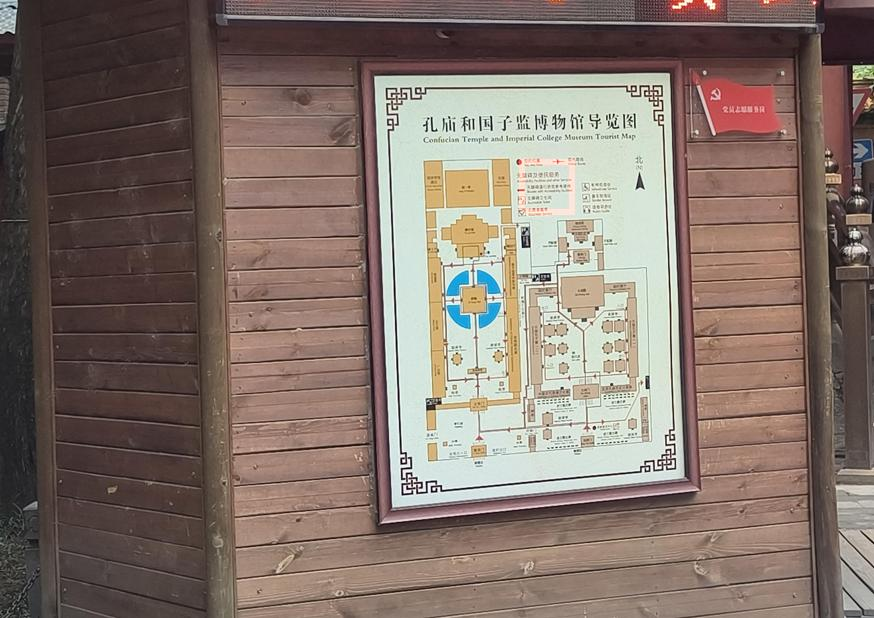}
       \includegraphics[width=.98\textwidth]{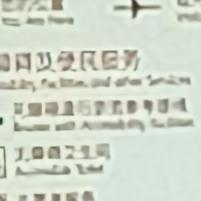}
       \includegraphics[width=.98\textwidth]{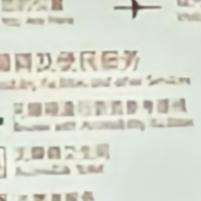}
    %    \includegraphics[width=.98\textwidth]{./compare/gt/336_crop.jpg}
        % \vspace{-6pt}
        \caption*{EDSR}
    \end{minipage}
    \begin{minipage}[b]{0.138\textwidth}
        \centering
        \setlength{\abovecaptionskip}{0.005cm}
       % \includegraphics[width=.98\textwidth]{./compare/Real_ESRGAN/615.jpg}
       % \includegraphics[width=.98\textwidth]{./compare/Real_ESRGAN/615_crop.jpg}
       % \includegraphics[width=.98\textwidth]{./compare/Real_ESRGAN-fin/615_crop.jpg}
    %    \includegraphics[width=.98\textwidth]{./compare/gt/615_crop.jpg}
    %    \caption*{Real_ESRGAN}
       \includegraphics[width=.98\textwidth]{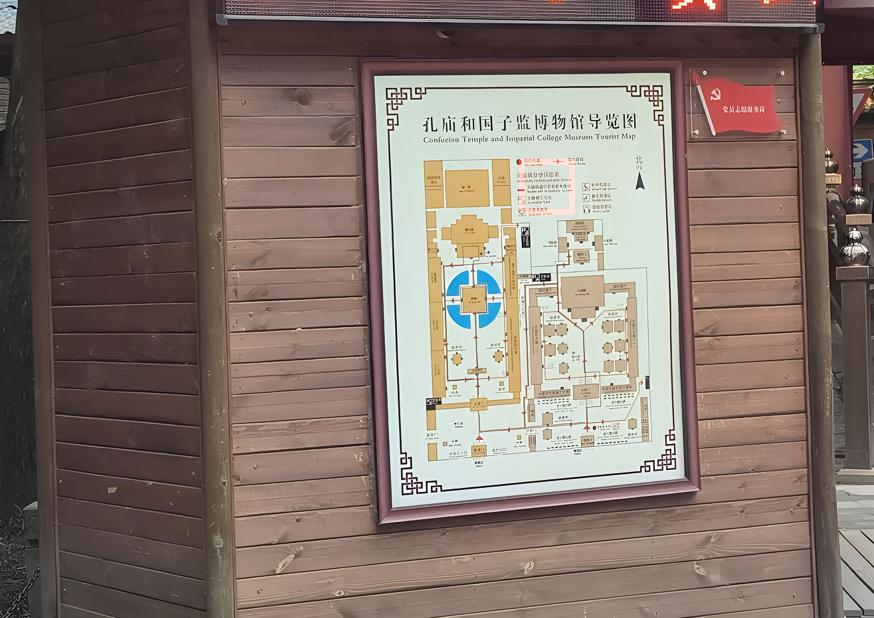}
       \includegraphics[width=.98\textwidth]{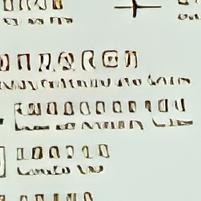}
       \includegraphics[width=.98\textwidth]{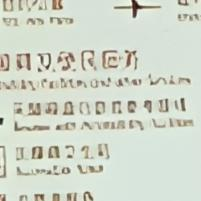}
    %    \includegraphics[width=.98\textwidth]{./compare/gt/336_crop.jpg}
        % \vspace{-6pt}
        \caption*{Real-ESRGAN}
    \end{minipage}
    \begin{minipage}[b]{0.138\textwidth}
        \centering
        \setlength{\abovecaptionskip}{0.005cm}
       % \includegraphics[width=.98\textwidth]{./compare/swinir/615.jpg}
       % \includegraphics[width=.98\textwidth]{./compare/swinir/615_crop.jpg}
       % \includegraphics[width=.98\textwidth]{./compare/swinir-fin/615_crop.jpg}
    %    \includegraphics[width=.98\textwidth]{./compare/gt/615_crop.jpg}
    %    \caption*{SwinIR}
       \includegraphics[width=.98\textwidth]{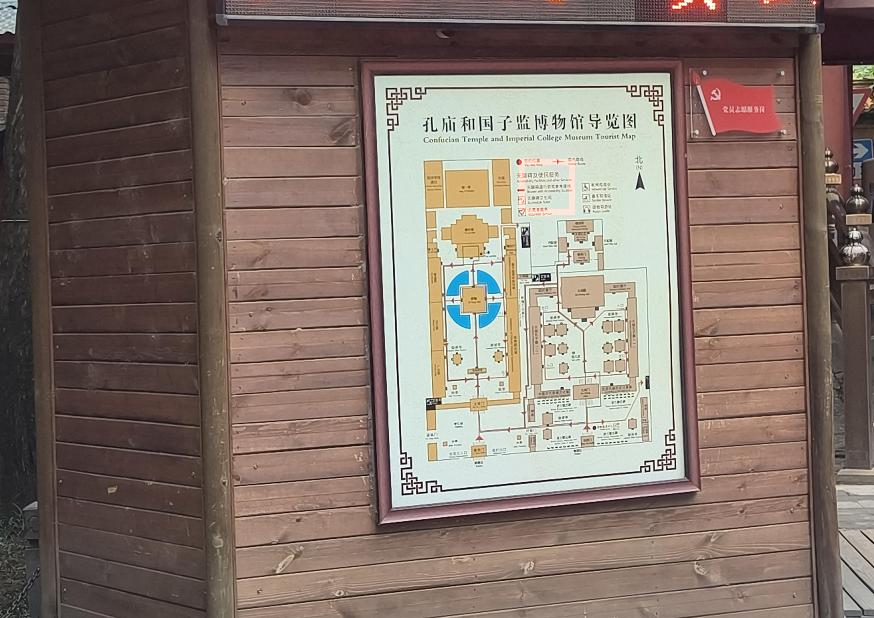}
       \includegraphics[width=.98\textwidth]{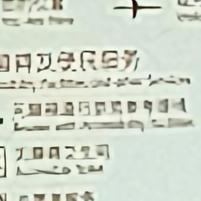}
       \includegraphics[width=.98\textwidth]{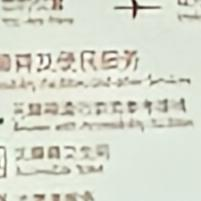}
    %    \includegraphics[width=.98\textwidth]{./compare/gt/336_crop.jpg}
        % \vspace{-6pt}
        \caption*{SwinIR}
    \end{minipage}
    \begin{minipage}[b]{0.138\textwidth}
        \centering
        \setlength{\abovecaptionskip}{0.005cm}
       % \includegraphics[width=.98\textwidth]{./compare/gt/615.jpg}
    %    \includegraphics[width=.98\textwidth]{./compare/swinir/615_crop.jpg}
    %    \includegraphics[width=.98\textwidth]{./compare/swinir-fin/615_crop.jpg}
       % \includegraphics[width=.98\textwidth]{./compare/gt/615_crop.jpg}
    %    \caption*{SwinIR}
       \includegraphics[width=.98\textwidth]{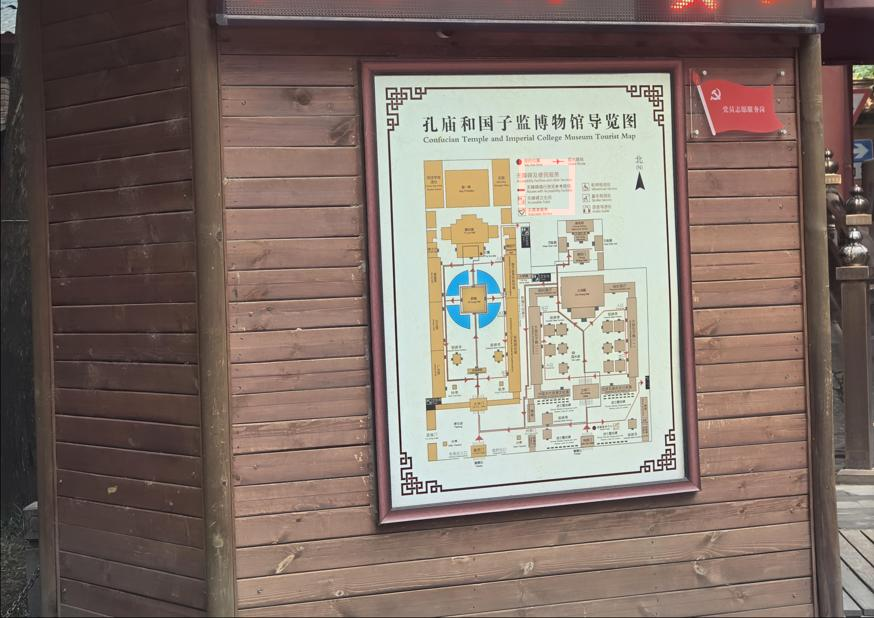}
       \includegraphics[width=.98\textwidth]{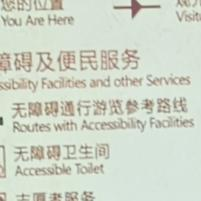}
       \includegraphics[width=.98\textwidth]{./compare/gt/336_crop.jpg}
        % \vspace{-6pt}
        \caption*{GT}
    \end{minipage}
    \vspace{-10pt}
    \caption{Example results of different algorithms trained on CameraFusion vs. ReWiTe. Top: The full-image results of different algorithms trained on ReWiTe. Middle: Results focused on the red-box region, derived from algorithms trained on CameraFusion. Bottom: Results focused on the red-box region, derived from algorithms trained on ReWiTe. Since the difficulty of perceiving differences of full-image results in compressed image size, only one full-image result is shown in the top line.
    }
    \label{fig: result compare4}
\end{figure*}

\begin{figure*}
    \centering
    \begin{minipage}[b]{0.138\textwidth}
        \centering
        \setlength{\abovecaptionskip}{0.005cm}
       % \includegraphics[width=.98\textwidth]{./compare/dcsr/615.jpg}
       % \includegraphics[width=.98\textwidth]{./compare/dcsr/615_crop.jpg}
       % \includegraphics[width=.98\textwidth]{./compare/dcsr-fin/615_crop.jpg}
    %    \includegraphics[width=.98\textwidth]{./compare/gt/615_crop.jpg}
    %    \caption*{srntt}
       \includegraphics[width=.98\textwidth]{./compare/tele/347.jpg}
       \includegraphics[width=.98\textwidth]{./compare/tele/347_crop.jpg}
       \includegraphics[width=.98\textwidth]{./compare/tele/347_crop.jpg}
       % \includegraphics[width=.98\textwidth]{./compare/tele/347_crop.jpg}
    %    \includegraphics[width=.98\textwidth]{./compare/gt/347_crop.jpg}
        % \vspace{-6pt}
        \caption*{\bf{Input T}}
    \end{minipage}
    \begin{minipage}[b]{0.138\textwidth}
    \centering
        \setlength{\abovecaptionskip}{0.005cm}
       % \includegraphics[width=.98\textwidth]{./compare/dcsr/615.jpg}
       % \includegraphics[width=.98\textwidth]{./compare/dcsr/615_crop.jpg}
       % \includegraphics[width=.98\textwidth]{./compare/dcsr-fin/615_crop.jpg}
    %    \includegraphics[width=.98\textwidth]{./compare/gt/615_crop.jpg}
    %    \caption*{srntt}
       \includegraphics[width=.98\textwidth]{./compare/w+t/347.jpg}
       \includegraphics[width=.98\textwidth]{./compare/w+t/347_crop.jpg}
       \includegraphics[width=.98\textwidth]{./compare/w+t/347_crop.jpg}
       % \includegraphics[width=.98\textwidth]{./compare/tele/347_crop.jpg}
    %    \includegraphics[width=.98\textwidth]{./compare/gt/347_crop.jpg}
        % \vspace{-6pt}
        \caption*{\bf{Input W}}
    \end{minipage}
    \begin{minipage}[b]{0.138\textwidth}
        \centering
        \setlength{\abovecaptionskip}{0.005cm}
       % \includegraphics[width=.98\textwidth]{./compare/dcsr/615.jpg}
       % \includegraphics[width=.98\textwidth]{./compare/dcsr/615_crop.jpg}
       % \includegraphics[width=.98\textwidth]{./compare/dcsr-fin/615_crop.jpg}
    %    \includegraphics[width=.98\textwidth]{./compare/gt/615_crop.jpg}
    %    \caption*{srntt}
       \includegraphics[width=.98\textwidth]{./compare/c2/347.jpg}
       \includegraphics[width=.98\textwidth]{./compare/c2/347_crop.jpg}
       \includegraphics[width=.98\textwidth]{./compare/c2-fin/347_crop.jpg}
    %    \includegraphics[width=.98\textwidth]{./compare/gt/347_crop.jpg}
        % \vspace{-6pt}
        \caption*{C2-matching}
    \end{minipage}
    \begin{minipage}[b]{0.138\textwidth}
        \centering
        \setlength{\abovecaptionskip}{0.005cm}
       % \includegraphics[width=.98\textwidth]{./compare/dcsr/615.jpg}
       % \includegraphics[width=.98\textwidth]{./compare/dcsr/615_crop.jpg}
       % \includegraphics[width=.98\textwidth]{./compare/dcsr-fin/615_crop.jpg}
    %    \includegraphics[width=.98\textwidth]{./compare/gt/615_crop.jpg}
    %    \caption*{srntt}
       \includegraphics[width=.98\textwidth]{./compare/dcsr/347.jpg}
       \includegraphics[width=.98\textwidth]{./compare/dcsr/347_crop.jpg}
       \includegraphics[width=.98\textwidth]{./compare/dcsr-fin/347_crop.jpg}
    %    \includegraphics[width=.98\textwidth]{./compare/gt/347_crop.jpg}
        % \vspace{-6pt}
        \caption*{DCSR}
    \end{minipage}
    \begin{minipage}[b]{0.138\textwidth}
        \centering
        \setlength{\abovecaptionskip}{0.005cm}
       % \includegraphics[width=.98\textwidth]{./compare/selfdzsr/615.jpg}
       % \includegraphics[width=.98\textwidth]{./compare/selfdzsr/615_crop.jpg}
       % \includegraphics[width=.98\textwidth]{./compare/selfdzsr-fin/615_crop.jpg}
    %    \includegraphics[width=.98\textwidth]{./compare/gt/615_crop.jpg}
    %    \caption*{srntt}
       \includegraphics[width=.98\textwidth]{./compare/selfdzsr/347.jpg}
       \includegraphics[width=.98\textwidth]{./compare/selfdzsr/347_crop.jpg}
       \includegraphics[width=.98\textwidth]{./compare/selfdzsr-fin/347_crop.jpg}
    %    \includegraphics[width=.98\textwidth]{./compare/gt/347_crop.jpg}
        % \vspace{-6pt}
        \caption*{SelfDZSR}
    \end{minipage}
    \begin{minipage}[b]{0.138\textwidth}
        \centering
        \setlength{\abovecaptionskip}{0.005cm}
       % \includegraphics[width=.98\textwidth]{./compare/zedusr/615.jpg}
       % \includegraphics[width=.98\textwidth]{./compare/zedusr/615_crop.jpg}
       % \includegraphics[width=.98\textwidth]{./compare/zedusr-fin/615_crop.jpg}
    %    \includegraphics[width=.98\textwidth]{./compare/gt/615_crop.jpg}
    %    \caption*{srntt}
       \includegraphics[width=.98\textwidth]{./compare/zedusr/347.jpg}
       \includegraphics[width=.98\textwidth]{./compare/zedusr/347_crop.jpg}
       \includegraphics[width=.98\textwidth]{./compare/zedusr-fin/347_crop.jpg}
    %    \includegraphics[width=.98\textwidth]{./compare/gt/347_crop.jpg}
        % \vspace{-6pt}
        \caption*{ZeDUSR}
    \end{minipage}
    \begin{minipage}[b]{0.138\textwidth}
        \centering
        \setlength{\abovecaptionskip}{0.005cm}
       % \includegraphics[width=.98\textwidth]{./compare/MASA/615.jpg}
       % \includegraphics[width=.98\textwidth]{./compare/MASA/615_crop.jpg}
       % \includegraphics[width=.98\textwidth]{./compare/MASA-fin/615_crop.jpg}
    %    \includegraphics[width=.98\textwidth]{./compare/gt/615_crop.jpg}
    %    \caption*{srntt}
       \includegraphics[width=.98\textwidth]{./compare/MASA/347.jpg}
       \includegraphics[width=.98\textwidth]{./compare/MASA/347_crop.jpg}
       \includegraphics[width=.98\textwidth]{./compare/MASA-fin/347_crop.jpg}
    %    \includegraphics[width=.98\textwidth]{./compare/gt/347_crop.jpg}
        % \vspace{-6pt}
        \caption*{MASA}
    \end{minipage}
    \begin{minipage}[b]{0.138\textwidth}
        \centering
        \setlength{\abovecaptionskip}{0.005cm}
       % \includegraphics[width=.98\textwidth]{./compare/ttsr/615.jpg}
       % \includegraphics[width=.98\textwidth]{./compare/ttsr/615_crop.jpg}
       % \includegraphics[width=.98\textwidth]{./compare/ttsr-fin/615_crop.jpg}
    %    \includegraphics[width=.98\textwidth]{./compare/gt/615_crop.jpg}
    %    \caption*{srntt}
       \includegraphics[width=.98\textwidth]{./compare/ttsr/347.jpg}
       \includegraphics[width=.98\textwidth]{./compare/ttsr/347_crop.jpg}
       \includegraphics[width=.98\textwidth]{./compare/ttsr-fin/347_crop.jpg}
    %    \includegraphics[width=.98\textwidth]{./compare/gt/347_crop.jpg}
        % \vspace{-6pt}
        \caption*{TTSR}
    \end{minipage}
    \begin{minipage}[b]{0.138\textwidth}
        \centering
        \setlength{\abovecaptionskip}{0.005cm}
       % \includegraphics[width=.98\textwidth]{./compare/srntt/615.jpg}
       % \includegraphics[width=.98\textwidth]{./compare/srntt/615_crop.jpg}
       % \includegraphics[width=.98\textwidth]{./compare/srntt-fin/615_crop.jpg}
    %    \includegraphics[width=.98\textwidth]{./compare/gt/615_crop.jpg}
    %    \caption*{srntt}
       \includegraphics[width=.98\textwidth]{./compare/srntt/347.jpg}
       \includegraphics[width=.98\textwidth]{./compare/srntt/347_crop.jpg}
       \includegraphics[width=.98\textwidth]{./compare/srntt-fin/347_crop.jpg}
    %    \includegraphics[width=.98\textwidth]{./compare/gt/347_crop.jpg}
        % \vspace{-6pt}
        \caption*{SRNTT}
    \end{minipage}
    \begin{minipage}[b]{0.138\textwidth}
        \centering
        \setlength{\abovecaptionskip}{0.005cm}
       % \includegraphics[width=.98\textwidth]{./compare/RCAN/615.jpg}
       % \includegraphics[width=.98\textwidth]{./compare/RCAN/615_crop.jpg}
       % \includegraphics[width=.98\textwidth]{./compare/RCAN-fin/615_crop.jpg}
    %    \includegraphics[width=.98\textwidth]{./compare/gt/615_crop.jpg}
    %    \caption*{RCAN}
       \includegraphics[width=.98\textwidth]{./compare/RCAN/347.jpg}
       \includegraphics[width=.98\textwidth]{./compare/RCAN/347_crop.jpg}
       \includegraphics[width=.98\textwidth]{./compare/RCAN-fin/347_crop.jpg}
    %    \includegraphics[width=.98\textwidth]{./compare/gt/347_crop.jpg}
        % \vspace{-6pt}
        \caption*{RCAN}
    \end{minipage}
    \begin{minipage}[b]{0.138\textwidth}
        \centering
        \setlength{\abovecaptionskip}{0.005cm}
       % \includegraphics[width=.98\textwidth]{./compare/EDSR/615.jpg}
       % \includegraphics[width=.98\textwidth]{./compare/EDSR/615_crop.jpg}
       % \includegraphics[width=.98\textwidth]{./compare/EDSR-fin/615_crop.jpg}
    %    \includegraphics[width=.98\textwidth]{./compare/gt/615_crop.jpg}
    %    \caption*{EDSR}
       \includegraphics[width=.98\textwidth]{./compare/EDSR/347.jpg}
       \includegraphics[width=.98\textwidth]{./compare/EDSR/347_crop.jpg}
       \includegraphics[width=.98\textwidth]{./compare/EDSR-fin/347_crop.jpg}
    %    \includegraphics[width=.98\textwidth]{./compare/gt/347_crop.jpg}
        % \vspace{-6pt}
        \caption*{EDSR}
    \end{minipage}
    \begin{minipage}[b]{0.138\textwidth}
        \centering
        \setlength{\abovecaptionskip}{0.005cm}
       % \includegraphics[width=.98\textwidth]{./compare/Real_ESRGAN/615.jpg}
       % \includegraphics[width=.98\textwidth]{./compare/Real_ESRGAN/615_crop.jpg}
       % \includegraphics[width=.98\textwidth]{./compare/Real_ESRGAN-fin/615_crop.jpg}
    %    \includegraphics[width=.98\textwidth]{./compare/gt/615_crop.jpg}
    %    \caption*{Real_ESRGAN}
       \includegraphics[width=.98\textwidth]{./compare/Real_ESRGAN/347.jpg}
       \includegraphics[width=.98\textwidth]{./compare/Real_ESRGAN/347_crop.jpg}
       \includegraphics[width=.98\textwidth]{./compare/Real_ESRGAN-fin/347_crop.jpg}
    %    \includegraphics[width=.98\textwidth]{./compare/gt/347_crop.jpg}
        % \vspace{-6pt}
        \caption*{Real-ESRGAN}
    \end{minipage}
    \begin{minipage}[b]{0.138\textwidth}
        \centering
        \setlength{\abovecaptionskip}{0.005cm}
       % \includegraphics[width=.98\textwidth]{./compare/swinir/615.jpg}
       % \includegraphics[width=.98\textwidth]{./compare/swinir/615_crop.jpg}
       % \includegraphics[width=.98\textwidth]{./compare/swinir-fin/615_crop.jpg}
    %    \includegraphics[width=.98\textwidth]{./compare/gt/615_crop.jpg}
    %    \caption*{SwinIR}
       \includegraphics[width=.98\textwidth]{./compare/swinir/347.jpg}
       \includegraphics[width=.98\textwidth]{./compare/swinir/347_crop.jpg}
       \includegraphics[width=.98\textwidth]{./compare/swinir-fin/347_crop.jpg}
    %    \includegraphics[width=.98\textwidth]{./compare/gt/347_crop.jpg}
        % \vspace{-6pt}
        \caption*{SwinIR}
    \end{minipage}
    \begin{minipage}[b]{0.138\textwidth}
        \centering
        \setlength{\abovecaptionskip}{0.005cm}
       % \includegraphics[width=.98\textwidth]{./compare/gt/615.jpg}
    %    \includegraphics[width=.98\textwidth]{./compare/swinir/615_crop.jpg}
    %    \includegraphics[width=.98\textwidth]{./compare/swinir-fin/615_crop.jpg}
       % \includegraphics[width=.98\textwidth]{./compare/gt/615_crop.jpg}
    %    \caption*{SwinIR}
       \includegraphics[width=.98\textwidth]{./compare/gt/347.jpg}
       \includegraphics[width=.98\textwidth]{./compare/gt/347_crop.jpg}
       \includegraphics[width=.98\textwidth]{./compare/gt/347_crop.jpg}
        % \vspace{-6pt}
        \caption*{GT}
    \end{minipage}
    \vspace{-10pt}
    \caption{Example results of different algorithms trained on CameraFusion vs. ReWiTe. Top: The full-image results of different algorithms trained on ReWiTe. Middle: Results focused on the red-box region, derived from algorithms trained on CameraFusion. Bottom: Results focused on the red-box region, derived from algorithms trained on ReWiTe. Since the difficulty of perceiving differences of full-image results in compressed image size, only one full-image result is shown in the top line.
    }
    \label{fig: result compare5}
\end{figure*}

\begin{figure*}
    \centering
    \begin{minipage}[b]{0.138\textwidth}
        \centering
        \setlength{\abovecaptionskip}{0.005cm}
       % \includegraphics[width=.98\textwidth]{./compare/dcsr/615.jpg}
       % \includegraphics[width=.98\textwidth]{./compare/dcsr/615_crop.jpg}
       % \includegraphics[width=.98\textwidth]{./compare/dcsr-fin/615_crop.jpg}
    %    \includegraphics[width=.98\textwidth]{./compare/gt/615_crop.jpg}
    %    \caption*{srntt}
       \includegraphics[width=.98\textwidth]{./compare/tele/482.jpg}
       \includegraphics[width=.98\textwidth]{./compare/tele/482_crop.jpg}
       \includegraphics[width=.98\textwidth]{./compare/tele/482_crop.jpg}
       % \includegraphics[width=.98\textwidth]{./compare/tele/482_crop.jpg}
    %    \includegraphics[width=.98\textwidth]{./compare/gt/482_crop.jpg}
        % \vspace{-6pt}
        \caption*{\bf{Input T}}
    \end{minipage}
    \begin{minipage}[b]{0.138\textwidth}
    \centering
        \setlength{\abovecaptionskip}{0.005cm}
       % \includegraphics[width=.98\textwidth]{./compare/dcsr/615.jpg}
       % \includegraphics[width=.98\textwidth]{./compare/dcsr/615_crop.jpg}
       % \includegraphics[width=.98\textwidth]{./compare/dcsr-fin/615_crop.jpg}
    %    \includegraphics[width=.98\textwidth]{./compare/gt/615_crop.jpg}
    %    \caption*{srntt}
       \includegraphics[width=.98\textwidth]{./compare/w+t/482.jpg}
       \includegraphics[width=.98\textwidth]{./compare/w+t/482_crop.jpg}
       \includegraphics[width=.98\textwidth]{./compare/w+t/482_crop.jpg}
       % \includegraphics[width=.98\textwidth]{./compare/tele/482_crop.jpg}
    %    \includegraphics[width=.98\textwidth]{./compare/gt/482_crop.jpg}
        % \vspace{-6pt}
        \caption*{\bf{Input W}}
    \end{minipage}
    \begin{minipage}[b]{0.138\textwidth}
        \centering
        \setlength{\abovecaptionskip}{0.005cm}
       % \includegraphics[width=.98\textwidth]{./compare/dcsr/615.jpg}
       % \includegraphics[width=.98\textwidth]{./compare/dcsr/615_crop.jpg}
       % \includegraphics[width=.98\textwidth]{./compare/dcsr-fin/615_crop.jpg}
    %    \includegraphics[width=.98\textwidth]{./compare/gt/615_crop.jpg}
    %    \caption*{srntt}
       \includegraphics[width=.98\textwidth]{./compare/c2/482.jpg}
       \includegraphics[width=.98\textwidth]{./compare/c2/482_crop.jpg}
       \includegraphics[width=.98\textwidth]{./compare/c2-fin/482_crop.jpg}
    %    \includegraphics[width=.98\textwidth]{./compare/gt/482_crop.jpg}
        % \vspace{-6pt}
        \caption*{C2-matching}
    \end{minipage}
    \begin{minipage}[b]{0.138\textwidth}
        \centering
        \setlength{\abovecaptionskip}{0.005cm}
       % \includegraphics[width=.98\textwidth]{./compare/dcsr/615.jpg}
       % \includegraphics[width=.98\textwidth]{./compare/dcsr/615_crop.jpg}
       % \includegraphics[width=.98\textwidth]{./compare/dcsr-fin/615_crop.jpg}
    %    \includegraphics[width=.98\textwidth]{./compare/gt/615_crop.jpg}
    %    \caption*{srntt}
       \includegraphics[width=.98\textwidth]{./compare/dcsr/482.jpg}
       \includegraphics[width=.98\textwidth]{./compare/dcsr/482_crop.jpg}
       \includegraphics[width=.98\textwidth]{./compare/dcsr-fin/482_crop.jpg}
    %    \includegraphics[width=.98\textwidth]{./compare/gt/482_crop.jpg}
        % \vspace{-6pt}
        \caption*{DCSR}
    \end{minipage}
    \begin{minipage}[b]{0.138\textwidth}
        \centering
        \setlength{\abovecaptionskip}{0.005cm}
       % \includegraphics[width=.98\textwidth]{./compare/selfdzsr/615.jpg}
       % \includegraphics[width=.98\textwidth]{./compare/selfdzsr/615_crop.jpg}
       % \includegraphics[width=.98\textwidth]{./compare/selfdzsr-fin/615_crop.jpg}
    %    \includegraphics[width=.98\textwidth]{./compare/gt/615_crop.jpg}
    %    \caption*{srntt}
       \includegraphics[width=.98\textwidth]{./compare/selfdzsr/482.jpg}
       \includegraphics[width=.98\textwidth]{./compare/selfdzsr/482_crop.jpg}
       \includegraphics[width=.98\textwidth]{./compare/selfdzsr-fin/482_crop.jpg}
    %    \includegraphics[width=.98\textwidth]{./compare/gt/482_crop.jpg}
        % \vspace{-6pt}
        \caption*{SelfDZSR}
    \end{minipage}
    \begin{minipage}[b]{0.138\textwidth}
        \centering
        \setlength{\abovecaptionskip}{0.005cm}
       % \includegraphics[width=.98\textwidth]{./compare/zedusr/615.jpg}
       % \includegraphics[width=.98\textwidth]{./compare/zedusr/615_crop.jpg}
       % \includegraphics[width=.98\textwidth]{./compare/zedusr-fin/615_crop.jpg}
    %    \includegraphics[width=.98\textwidth]{./compare/gt/615_crop.jpg}
    %    \caption*{srntt}
       \includegraphics[width=.98\textwidth]{./compare/zedusr/482.jpg}
       \includegraphics[width=.98\textwidth]{./compare/zedusr/482_crop.jpg}
       \includegraphics[width=.98\textwidth]{./compare/zedusr-fin/482_crop.jpg}
    %    \includegraphics[width=.98\textwidth]{./compare/gt/482_crop.jpg}
        % \vspace{-6pt}
        \caption*{ZeDUSR}
    \end{minipage}
    \begin{minipage}[b]{0.138\textwidth}
        \centering
        \setlength{\abovecaptionskip}{0.005cm}
       % \includegraphics[width=.98\textwidth]{./compare/MASA/615.jpg}
       % \includegraphics[width=.98\textwidth]{./compare/MASA/615_crop.jpg}
       % \includegraphics[width=.98\textwidth]{./compare/MASA-fin/615_crop.jpg}
    %    \includegraphics[width=.98\textwidth]{./compare/gt/615_crop.jpg}
    %    \caption*{srntt}
       \includegraphics[width=.98\textwidth]{./compare/MASA/482.jpg}
       \includegraphics[width=.98\textwidth]{./compare/MASA/482_crop.jpg}
       \includegraphics[width=.98\textwidth]{./compare/MASA-fin/482_crop.jpg}
    %    \includegraphics[width=.98\textwidth]{./compare/gt/482_crop.jpg}
        % \vspace{-6pt}
        \caption*{MASA}
    \end{minipage}
    \begin{minipage}[b]{0.138\textwidth}
        \centering
        \setlength{\abovecaptionskip}{0.005cm}
       % \includegraphics[width=.98\textwidth]{./compare/ttsr/615.jpg}
       % \includegraphics[width=.98\textwidth]{./compare/ttsr/615_crop.jpg}
       % \includegraphics[width=.98\textwidth]{./compare/ttsr-fin/615_crop.jpg}
    %    \includegraphics[width=.98\textwidth]{./compare/gt/615_crop.jpg}
    %    \caption*{srntt}
       \includegraphics[width=.98\textwidth]{./compare/ttsr/482.jpg}
       \includegraphics[width=.98\textwidth]{./compare/ttsr/482_crop.jpg}
       \includegraphics[width=.98\textwidth]{./compare/ttsr-fin/482_crop.jpg}
    %    \includegraphics[width=.98\textwidth]{./compare/gt/482_crop.jpg}
        % \vspace{-6pt}
        \caption*{TTSR}
    \end{minipage}
    \begin{minipage}[b]{0.138\textwidth}
        \centering
        \setlength{\abovecaptionskip}{0.005cm}
       % \includegraphics[width=.98\textwidth]{./compare/srntt/615.jpg}
       % \includegraphics[width=.98\textwidth]{./compare/srntt/615_crop.jpg}
       % \includegraphics[width=.98\textwidth]{./compare/srntt-fin/615_crop.jpg}
    %    \includegraphics[width=.98\textwidth]{./compare/gt/615_crop.jpg}
    %    \caption*{srntt}
       \includegraphics[width=.98\textwidth]{./compare/srntt/482.jpg}
       \includegraphics[width=.98\textwidth]{./compare/srntt/482_crop.jpg}
       \includegraphics[width=.98\textwidth]{./compare/srntt-fin/482_crop.jpg}
    %    \includegraphics[width=.98\textwidth]{./compare/gt/482_crop.jpg}
        % \vspace{-6pt}
        \caption*{SRNTT}
    \end{minipage}
    \begin{minipage}[b]{0.138\textwidth}
        \centering
        \setlength{\abovecaptionskip}{0.005cm}
       % \includegraphics[width=.98\textwidth]{./compare/RCAN/615.jpg}
       % \includegraphics[width=.98\textwidth]{./compare/RCAN/615_crop.jpg}
       % \includegraphics[width=.98\textwidth]{./compare/RCAN-fin/615_crop.jpg}
    %    \includegraphics[width=.98\textwidth]{./compare/gt/615_crop.jpg}
    %    \caption*{RCAN}
       \includegraphics[width=.98\textwidth]{./compare/RCAN/482.jpg}
       \includegraphics[width=.98\textwidth]{./compare/RCAN/482_crop.jpg}
       \includegraphics[width=.98\textwidth]{./compare/RCAN-fin/482_crop.jpg}
    %    \includegraphics[width=.98\textwidth]{./compare/gt/482_crop.jpg}
        % \vspace{-6pt}
        \caption*{RCAN}
    \end{minipage}
    \begin{minipage}[b]{0.138\textwidth}
        \centering
        \setlength{\abovecaptionskip}{0.005cm}
       % \includegraphics[width=.98\textwidth]{./compare/EDSR/615.jpg}
       % \includegraphics[width=.98\textwidth]{./compare/EDSR/615_crop.jpg}
       % \includegraphics[width=.98\textwidth]{./compare/EDSR-fin/615_crop.jpg}
    %    \includegraphics[width=.98\textwidth]{./compare/gt/615_crop.jpg}
    %    \caption*{EDSR}
       \includegraphics[width=.98\textwidth]{./compare/EDSR/482.jpg}
       \includegraphics[width=.98\textwidth]{./compare/EDSR/482_crop.jpg}
       \includegraphics[width=.98\textwidth]{./compare/EDSR-fin/482_crop.jpg}
    %    \includegraphics[width=.98\textwidth]{./compare/gt/482_crop.jpg}
        % \vspace{-6pt}
        \caption*{EDSR}
    \end{minipage}
    \begin{minipage}[b]{0.138\textwidth}
        \centering
        \setlength{\abovecaptionskip}{0.005cm}
       % \includegraphics[width=.98\textwidth]{./compare/Real_ESRGAN/615.jpg}
       % \includegraphics[width=.98\textwidth]{./compare/Real_ESRGAN/615_crop.jpg}
       % \includegraphics[width=.98\textwidth]{./compare/Real_ESRGAN-fin/615_crop.jpg}
    %    \includegraphics[width=.98\textwidth]{./compare/gt/615_crop.jpg}
    %    \caption*{Real_ESRGAN}
       \includegraphics[width=.98\textwidth]{./compare/Real_ESRGAN/482.jpg}
       \includegraphics[width=.98\textwidth]{./compare/Real_ESRGAN/482_crop.jpg}
       \includegraphics[width=.98\textwidth]{./compare/Real_ESRGAN-fin/482_crop.jpg}
    %    \includegraphics[width=.98\textwidth]{./compare/gt/482_crop.jpg}
        % \vspace{-6pt}
        \caption*{Real-ESRGAN}
    \end{minipage}
    \begin{minipage}[b]{0.138\textwidth}
        \centering
        \setlength{\abovecaptionskip}{0.005cm}
       % \includegraphics[width=.98\textwidth]{./compare/swinir/615.jpg}
       % \includegraphics[width=.98\textwidth]{./compare/swinir/615_crop.jpg}
       % \includegraphics[width=.98\textwidth]{./compare/swinir-fin/615_crop.jpg}
    %    \includegraphics[width=.98\textwidth]{./compare/gt/615_crop.jpg}
    %    \caption*{SwinIR}
       \includegraphics[width=.98\textwidth]{./compare/swinir/482.jpg}
       \includegraphics[width=.98\textwidth]{./compare/swinir/482_crop.jpg}
       \includegraphics[width=.98\textwidth]{./compare/swinir-fin/482_crop.jpg}
    %    \includegraphics[width=.98\textwidth]{./compare/gt/482_crop.jpg}
        % \vspace{-6pt}
        \caption*{SwinIR}
    \end{minipage}
    \begin{minipage}[b]{0.138\textwidth}
        \centering
        \setlength{\abovecaptionskip}{0.005cm}
       % \includegraphics[width=.98\textwidth]{./compare/gt/615.jpg}
    %    \includegraphics[width=.98\textwidth]{./compare/swinir/615_crop.jpg}
    %    \includegraphics[width=.98\textwidth]{./compare/swinir-fin/615_crop.jpg}
       % \includegraphics[width=.98\textwidth]{./compare/gt/615_crop.jpg}
    %    \caption*{SwinIR}
       \includegraphics[width=.98\textwidth]{./compare/gt/482.jpg}
       \includegraphics[width=.98\textwidth]{./compare/gt/482_crop.jpg}
       \includegraphics[width=.98\textwidth]{./compare/gt/482_crop.jpg}
        % \vspace{-6pt}
        \caption*{GT}
    \end{minipage}
    \vspace{-10pt}
    \caption{Example results of different algorithms trained on CameraFusion vs. ReWiTe. Top: The full-image results of different algorithms trained on ReWiTe. Middle: Results focused on the red-box region, derived from algorithms trained on CameraFusion. Bottom: Results focused on the red-box region, derived from algorithms trained on ReWiTe. Since the difficulty of perceiving differences of full-image results in compressed image size, only one full-image result is shown in the top line.
    }
    \label{fig: result compare9}
\end{figure*}

\begin{figure*}
    \centering
    \begin{minipage}[b]{0.138\textwidth}
        \centering
        \setlength{\abovecaptionskip}{0.005cm}
       % \includegraphics[width=.98\textwidth]{./compare/dcsr/615.jpg}
       % \includegraphics[width=.98\textwidth]{./compare/dcsr/615_crop.jpg}
       % \includegraphics[width=.98\textwidth]{./compare/dcsr-fin/615_crop.jpg}
    %    \includegraphics[width=.98\textwidth]{./compare/gt/615_crop.jpg}
    %    \caption*{srntt}
       \includegraphics[width=.98\textwidth]{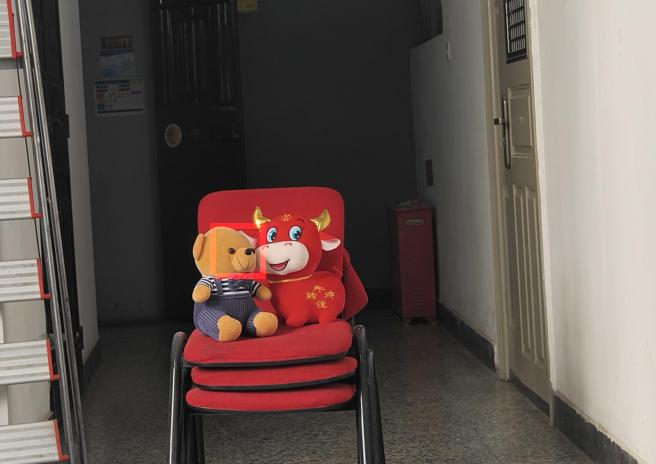}
       \includegraphics[width=.98\textwidth]{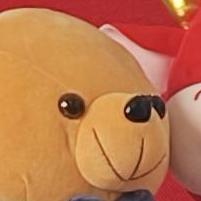}
       \includegraphics[width=.98\textwidth]{./compare/tele/771_crop.jpg}
       % \includegraphics[width=.98\textwidth]{./compare/tele/771_crop.jpg}
    %    \includegraphics[width=.98\textwidth]{./compare/gt/771_crop.jpg}
        % \vspace{-6pt}
        \caption*{\bf{Input T}}
    \end{minipage}
    \begin{minipage}[b]{0.138\textwidth}
    \centering
        \setlength{\abovecaptionskip}{0.005cm}
       % \includegraphics[width=.98\textwidth]{./compare/dcsr/615.jpg}
       % \includegraphics[width=.98\textwidth]{./compare/dcsr/615_crop.jpg}
       % \includegraphics[width=.98\textwidth]{./compare/dcsr-fin/615_crop.jpg}
    %    \includegraphics[width=.98\textwidth]{./compare/gt/615_crop.jpg}
    %    \caption*{srntt}
       \includegraphics[width=.98\textwidth]{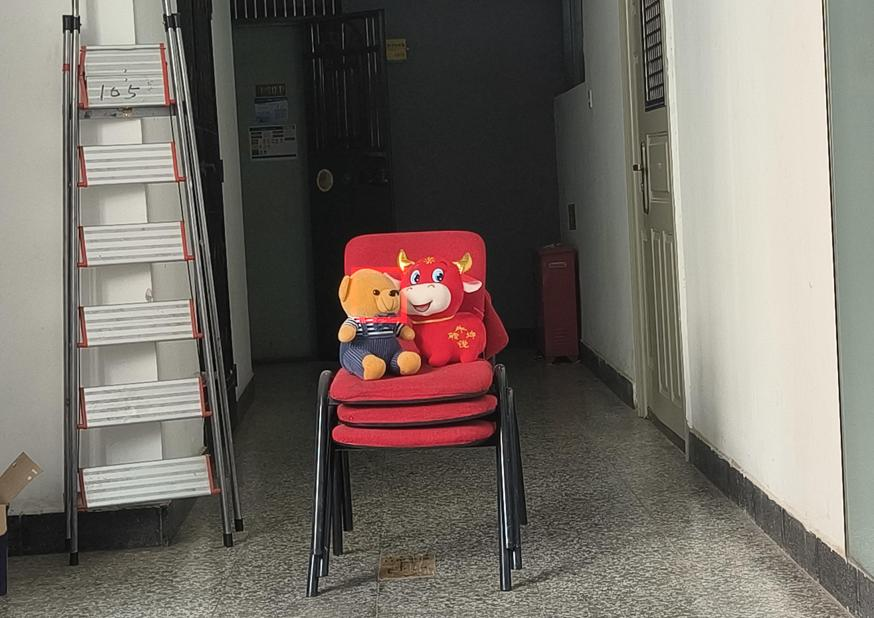}
       \includegraphics[width=.98\textwidth]{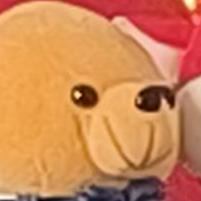}
       \includegraphics[width=.98\textwidth]{./compare/w+t/771_crop.jpg}
       % \includegraphics[width=.98\textwidth]{./compare/tele/771_crop.jpg}
    %    \includegraphics[width=.98\textwidth]{./compare/gt/771_crop.jpg}
        % \vspace{-6pt}
        \caption*{\bf{Input W}}
    \end{minipage}
    \begin{minipage}[b]{0.138\textwidth}
        \centering
        \setlength{\abovecaptionskip}{0.005cm}
       % \includegraphics[width=.98\textwidth]{./compare/dcsr/615.jpg}
       % \includegraphics[width=.98\textwidth]{./compare/dcsr/615_crop.jpg}
       % \includegraphics[width=.98\textwidth]{./compare/dcsr-fin/615_crop.jpg}
    %    \includegraphics[width=.98\textwidth]{./compare/gt/615_crop.jpg}
    %    \caption*{srntt}
       \includegraphics[width=.98\textwidth]{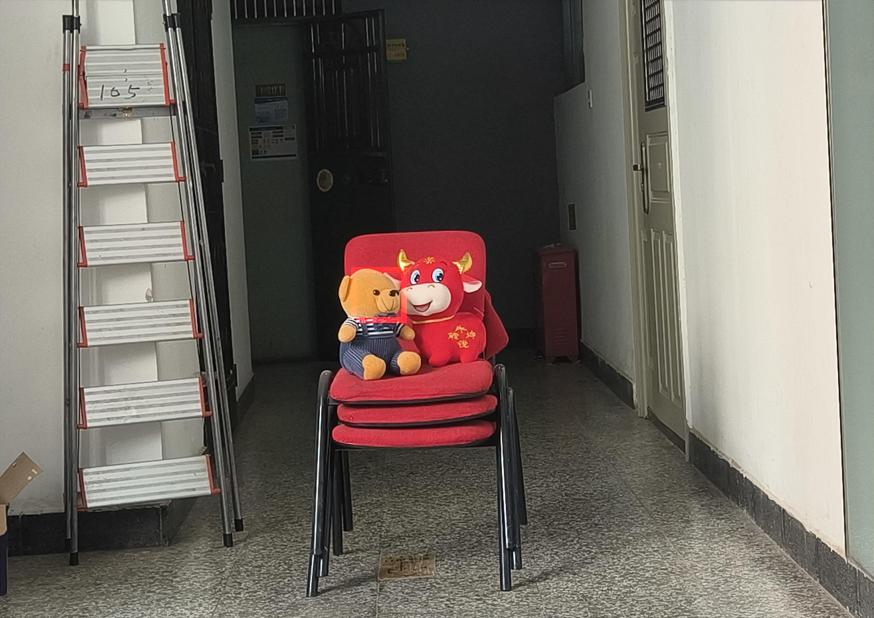}
       \includegraphics[width=.98\textwidth]{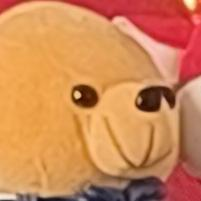}
       \includegraphics[width=.98\textwidth]{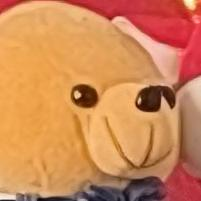}
    %    \includegraphics[width=.98\textwidth]{./compare/gt/771_crop.jpg}
        % \vspace{-6pt}
        \caption*{C2-matching}
    \end{minipage}
    \begin{minipage}[b]{0.138\textwidth}
        \centering
        \setlength{\abovecaptionskip}{0.005cm}
       % \includegraphics[width=.98\textwidth]{./compare/dcsr/615.jpg}
       % \includegraphics[width=.98\textwidth]{./compare/dcsr/615_crop.jpg}
       % \includegraphics[width=.98\textwidth]{./compare/dcsr-fin/615_crop.jpg}
    %    \includegraphics[width=.98\textwidth]{./compare/gt/615_crop.jpg}
    %    \caption*{srntt}
       \includegraphics[width=.98\textwidth]{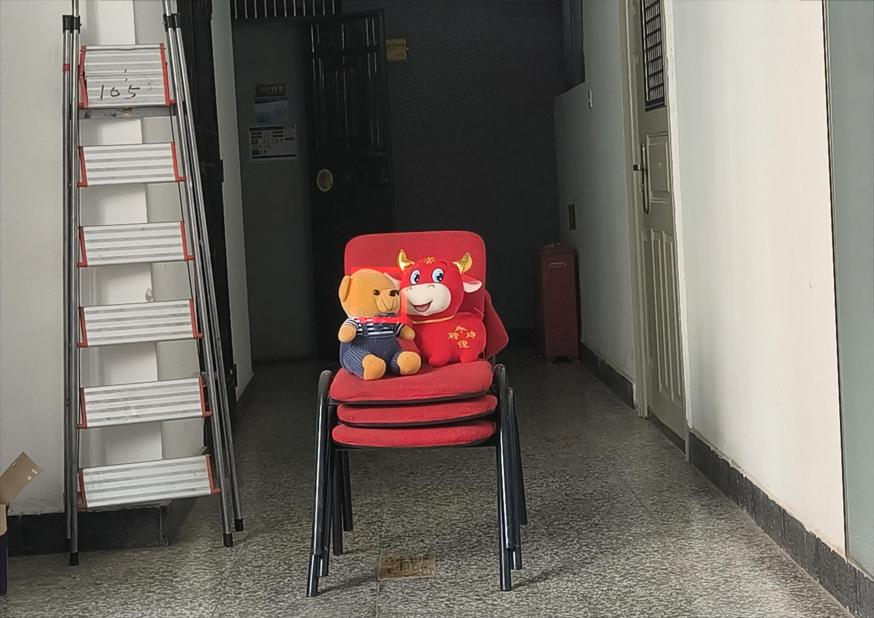}
       \includegraphics[width=.98\textwidth]{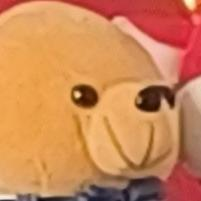}
       \includegraphics[width=.98\textwidth]{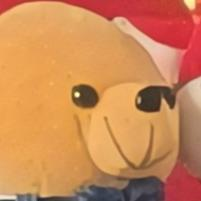}
    %    \includegraphics[width=.98\textwidth]{./compare/gt/771_crop.jpg}
        % \vspace{-6pt}
        \caption*{DCSR}
    \end{minipage}
    \begin{minipage}[b]{0.138\textwidth}
        \centering
        \setlength{\abovecaptionskip}{0.005cm}
       % \includegraphics[width=.98\textwidth]{./compare/selfdzsr/615.jpg}
       % \includegraphics[width=.98\textwidth]{./compare/selfdzsr/615_crop.jpg}
       % \includegraphics[width=.98\textwidth]{./compare/selfdzsr-fin/615_crop.jpg}
    %    \includegraphics[width=.98\textwidth]{./compare/gt/615_crop.jpg}
    %    \caption*{srntt}
       \includegraphics[width=.98\textwidth]{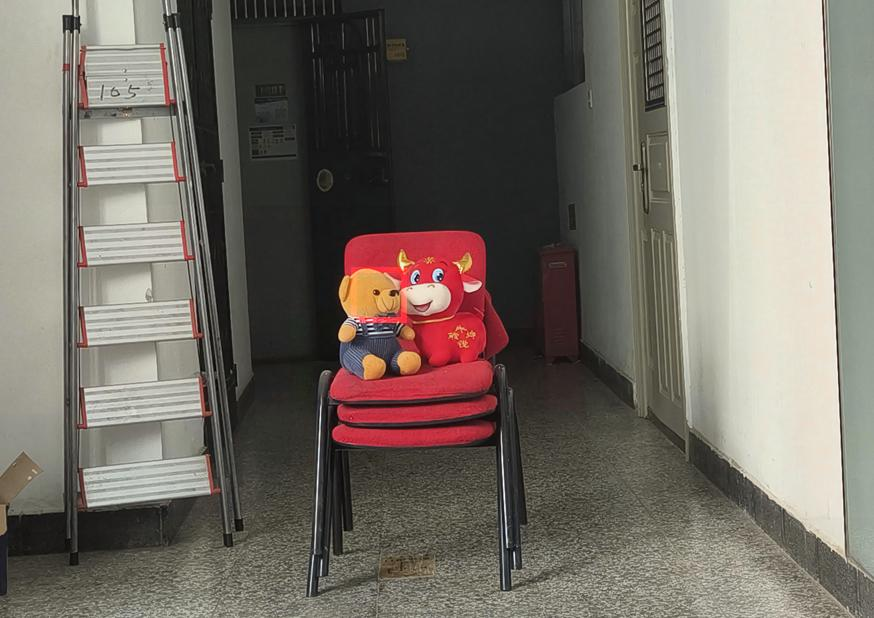}
       \includegraphics[width=.98\textwidth]{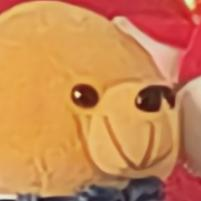}
       \includegraphics[width=.98\textwidth]{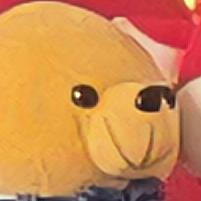}
    %    \includegraphics[width=.98\textwidth]{./compare/gt/771_crop.jpg}
        % \vspace{-6pt}
        \caption*{SelfDZSR}
    \end{minipage}
    \begin{minipage}[b]{0.138\textwidth}
        \centering
        \setlength{\abovecaptionskip}{0.005cm}
       % \includegraphics[width=.98\textwidth]{./compare/zedusr/615.jpg}
       % \includegraphics[width=.98\textwidth]{./compare/zedusr/615_crop.jpg}
       % \includegraphics[width=.98\textwidth]{./compare/zedusr-fin/615_crop.jpg}
    %    \includegraphics[width=.98\textwidth]{./compare/gt/615_crop.jpg}
    %    \caption*{srntt}
       \includegraphics[width=.98\textwidth]{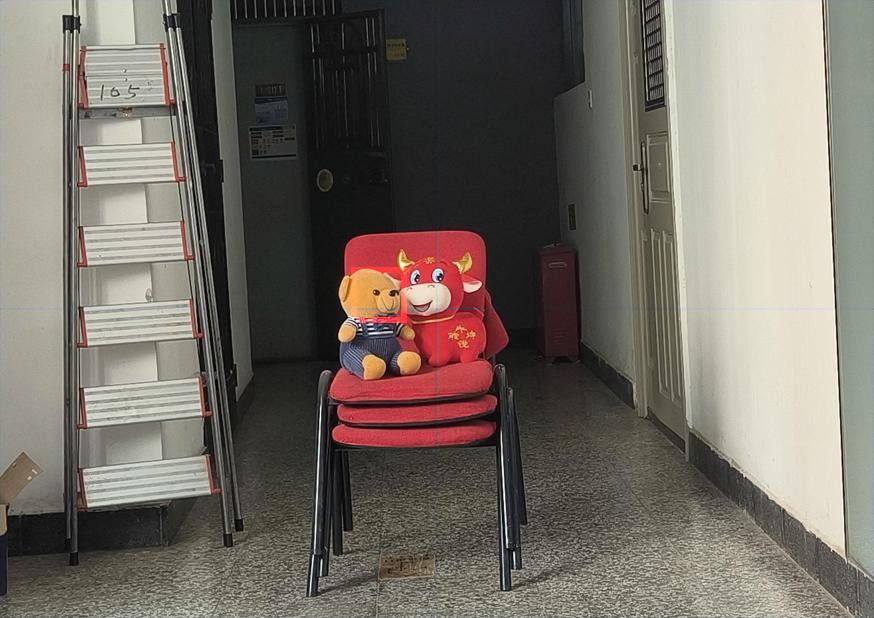}
       \includegraphics[width=.98\textwidth]{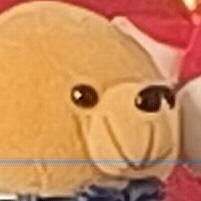}
       \includegraphics[width=.98\textwidth]{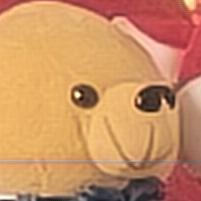}
    %    \includegraphics[width=.98\textwidth]{./compare/gt/771_crop.jpg}
        % \vspace{-6pt}
        \caption*{ZeDUSR}
    \end{minipage}
    \begin{minipage}[b]{0.138\textwidth}
        \centering
        \setlength{\abovecaptionskip}{0.005cm}
       % \includegraphics[width=.98\textwidth]{./compare/MASA/615.jpg}
       % \includegraphics[width=.98\textwidth]{./compare/MASA/615_crop.jpg}
       % \includegraphics[width=.98\textwidth]{./compare/MASA-fin/615_crop.jpg}
    %    \includegraphics[width=.98\textwidth]{./compare/gt/615_crop.jpg}
    %    \caption*{srntt}
       \includegraphics[width=.98\textwidth]{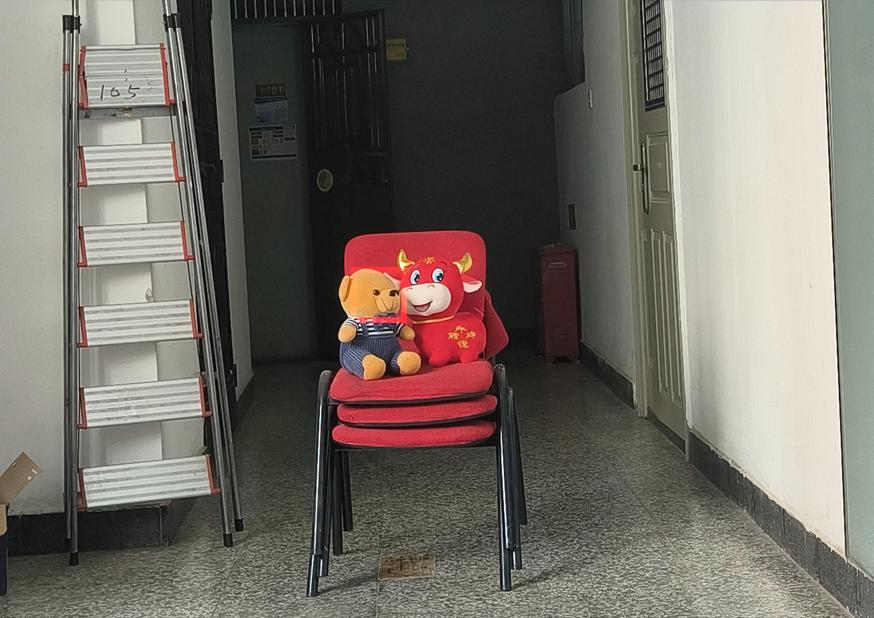}
       \includegraphics[width=.98\textwidth]{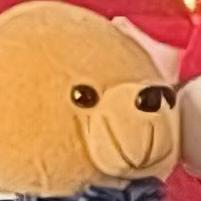}
       \includegraphics[width=.98\textwidth]{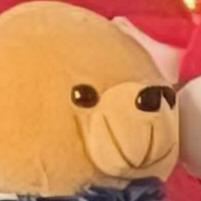}
    %    \includegraphics[width=.98\textwidth]{./compare/gt/771_crop.jpg}
        % \vspace{-6pt}
        \caption*{MASA}
    \end{minipage}
    \begin{minipage}[b]{0.138\textwidth}
        \centering
        \setlength{\abovecaptionskip}{0.005cm}
       % \includegraphics[width=.98\textwidth]{./compare/ttsr/615.jpg}
       % \includegraphics[width=.98\textwidth]{./compare/ttsr/615_crop.jpg}
       % \includegraphics[width=.98\textwidth]{./compare/ttsr-fin/615_crop.jpg}
    %    \includegraphics[width=.98\textwidth]{./compare/gt/615_crop.jpg}
    %    \caption*{srntt}
       \includegraphics[width=.98\textwidth]{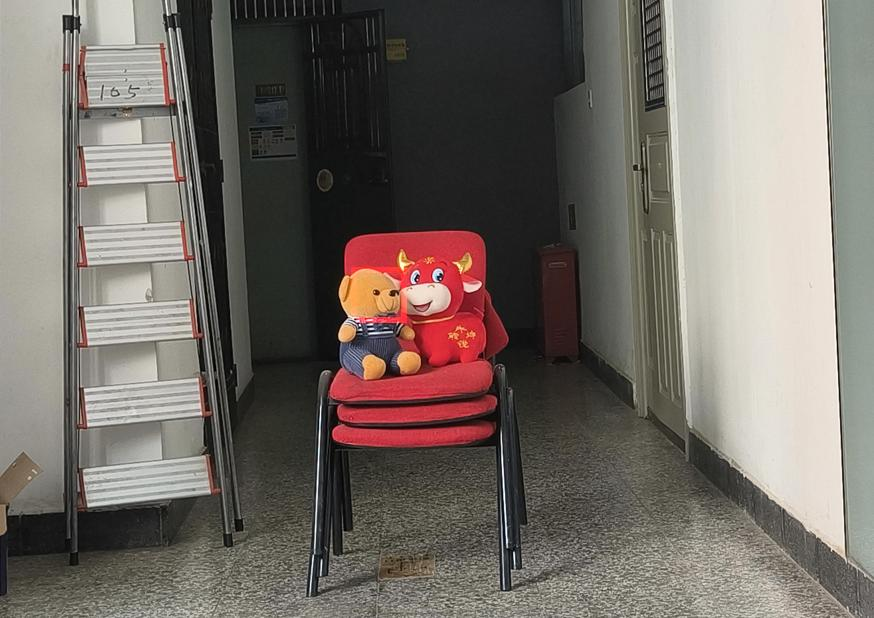}
       \includegraphics[width=.98\textwidth]{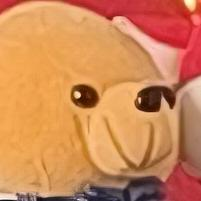}
       \includegraphics[width=.98\textwidth]{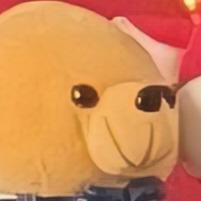}
    %    \includegraphics[width=.98\textwidth]{./compare/gt/771_crop.jpg}
        % \vspace{-6pt}
        \caption*{TTSR}
    \end{minipage}
    \begin{minipage}[b]{0.138\textwidth}
        \centering
        \setlength{\abovecaptionskip}{0.005cm}
       % \includegraphics[width=.98\textwidth]{./compare/srntt/615.jpg}
       % \includegraphics[width=.98\textwidth]{./compare/srntt/615_crop.jpg}
       % \includegraphics[width=.98\textwidth]{./compare/srntt-fin/615_crop.jpg}
    %    \includegraphics[width=.98\textwidth]{./compare/gt/615_crop.jpg}
    %    \caption*{srntt}
       \includegraphics[width=.98\textwidth]{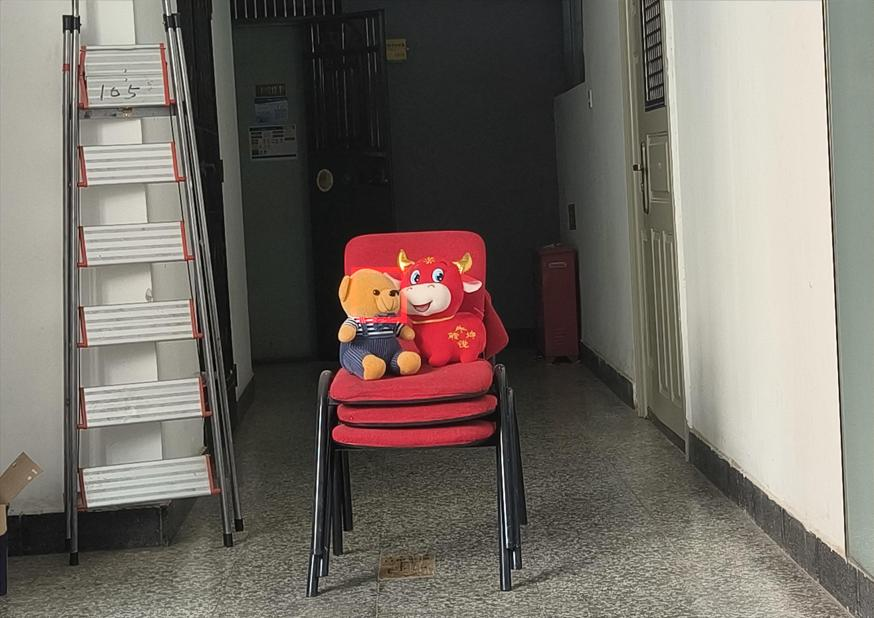}
       \includegraphics[width=.98\textwidth]{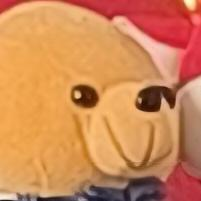}
       \includegraphics[width=.98\textwidth]{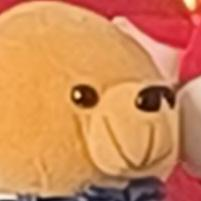}
    %    \includegraphics[width=.98\textwidth]{./compare/gt/771_crop.jpg}
        % \vspace{-6pt}
        \caption*{SRNTT}
    \end{minipage}
    \begin{minipage}[b]{0.138\textwidth}
        \centering
        \setlength{\abovecaptionskip}{0.005cm}
       % \includegraphics[width=.98\textwidth]{./compare/RCAN/615.jpg}
       % \includegraphics[width=.98\textwidth]{./compare/RCAN/615_crop.jpg}
       % \includegraphics[width=.98\textwidth]{./compare/RCAN-fin/615_crop.jpg}
    %    \includegraphics[width=.98\textwidth]{./compare/gt/615_crop.jpg}
    %    \caption*{RCAN}
       \includegraphics[width=.98\textwidth]{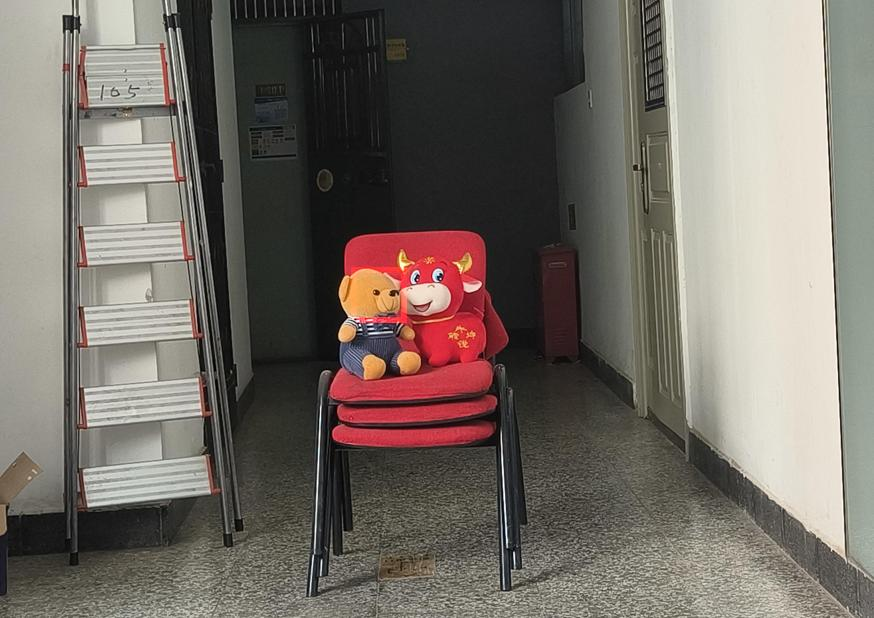}
       \includegraphics[width=.98\textwidth]{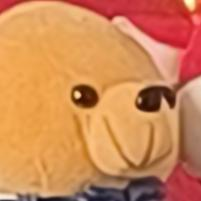}
       \includegraphics[width=.98\textwidth]{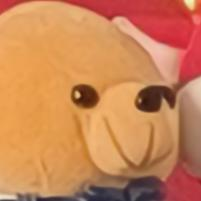}
    %    \includegraphics[width=.98\textwidth]{./compare/gt/771_crop.jpg}
        % \vspace{-6pt}
        \caption*{RCAN}
    \end{minipage}
    \begin{minipage}[b]{0.138\textwidth}
        \centering
        \setlength{\abovecaptionskip}{0.005cm}
       % \includegraphics[width=.98\textwidth]{./compare/EDSR/615.jpg}
       % \includegraphics[width=.98\textwidth]{./compare/EDSR/615_crop.jpg}
       % \includegraphics[width=.98\textwidth]{./compare/EDSR-fin/615_crop.jpg}
    %    \includegraphics[width=.98\textwidth]{./compare/gt/615_crop.jpg}
    %    \caption*{EDSR}
       \includegraphics[width=.98\textwidth]{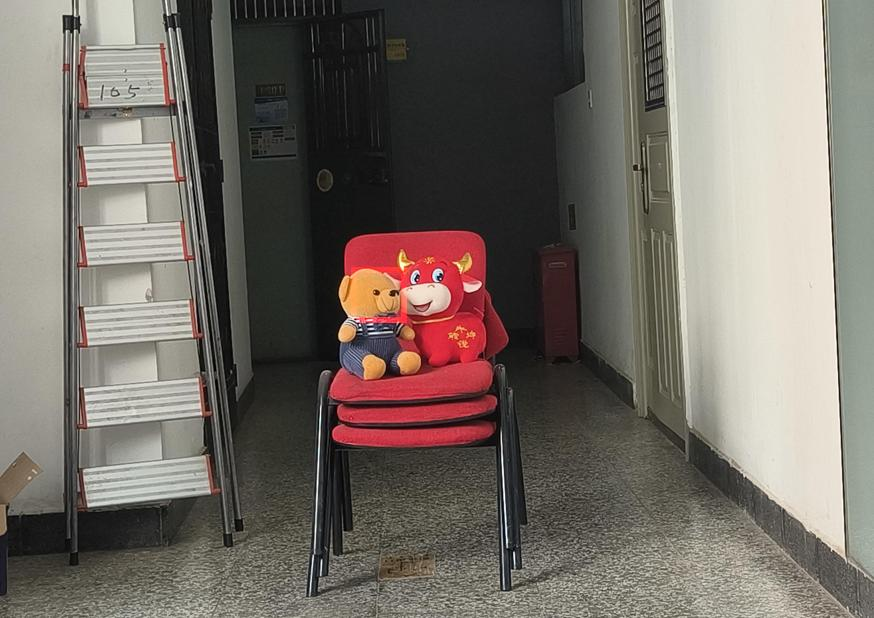}
       \includegraphics[width=.98\textwidth]{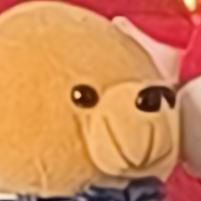}
       \includegraphics[width=.98\textwidth]{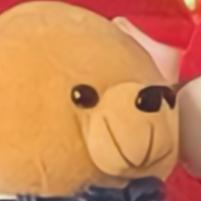}
    %    \includegraphics[width=.98\textwidth]{./compare/gt/771_crop.jpg}
        % \vspace{-6pt}
        \caption*{EDSR}
    \end{minipage}
    \begin{minipage}[b]{0.138\textwidth}
        \centering
        \setlength{\abovecaptionskip}{0.005cm}
       % \includegraphics[width=.98\textwidth]{./compare/Real_ESRGAN/615.jpg}
       % \includegraphics[width=.98\textwidth]{./compare/Real_ESRGAN/615_crop.jpg}
       % \includegraphics[width=.98\textwidth]{./compare/Real_ESRGAN-fin/615_crop.jpg}
    %    \includegraphics[width=.98\textwidth]{./compare/gt/615_crop.jpg}
    %    \caption*{Real_ESRGAN}
       \includegraphics[width=.98\textwidth]{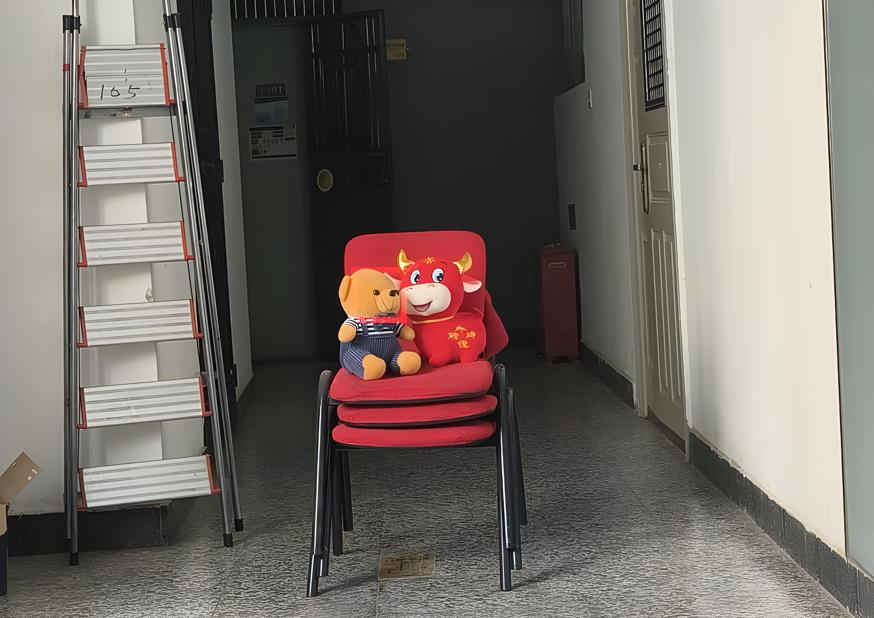}
       \includegraphics[width=.98\textwidth]{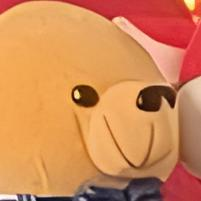}
       \includegraphics[width=.98\textwidth]{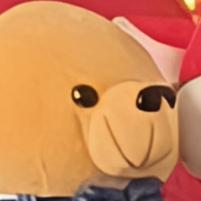}
    %    \includegraphics[width=.98\textwidth]{./compare/gt/771_crop.jpg}
        % \vspace{-6pt}
        \caption*{Real-ESRGAN}
    \end{minipage}
    \begin{minipage}[b]{0.138\textwidth}
        \centering
        \setlength{\abovecaptionskip}{0.005cm}
       % \includegraphics[width=.98\textwidth]{./compare/swinir/615.jpg}
       % \includegraphics[width=.98\textwidth]{./compare/swinir/615_crop.jpg}
       % \includegraphics[width=.98\textwidth]{./compare/swinir-fin/615_crop.jpg}
    %    \includegraphics[width=.98\textwidth]{./compare/gt/615_crop.jpg}
    %    \caption*{SwinIR}
       \includegraphics[width=.98\textwidth]{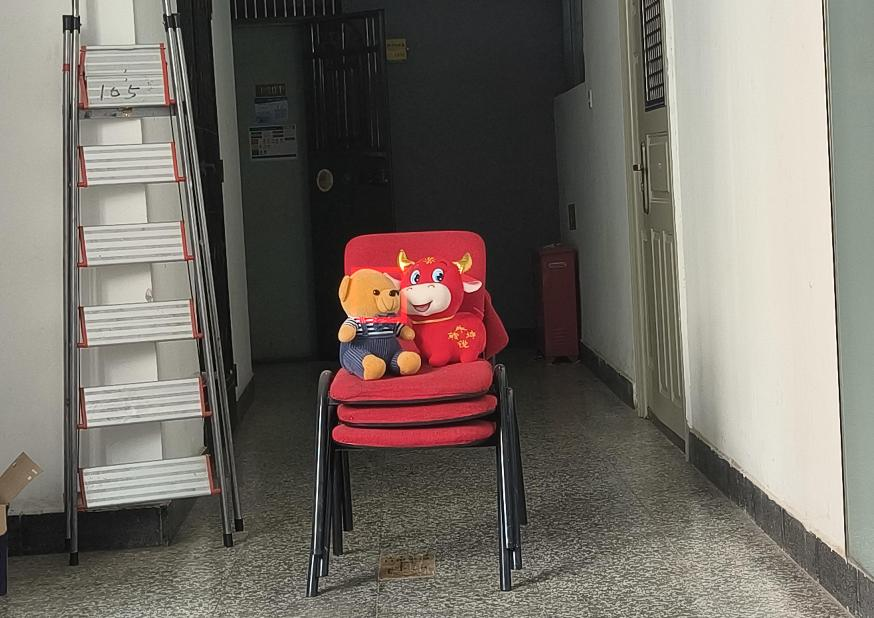}
       \includegraphics[width=.98\textwidth]{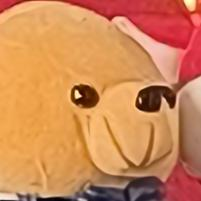}
       \includegraphics[width=.98\textwidth]{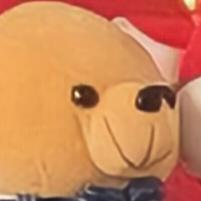}
    %    \includegraphics[width=.98\textwidth]{./compare/gt/771_crop.jpg}
        % \vspace{-6pt}
        \caption*{SwinIR}
    \end{minipage}
    \begin{minipage}[b]{0.138\textwidth}
        \centering
        \setlength{\abovecaptionskip}{0.005cm}
       % \includegraphics[width=.98\textwidth]{./compare/gt/615.jpg}
    %    \includegraphics[width=.98\textwidth]{./compare/swinir/615_crop.jpg}
    %    \includegraphics[width=.98\textwidth]{./compare/swinir-fin/615_crop.jpg}
       % \includegraphics[width=.98\textwidth]{./compare/gt/615_crop.jpg}
    %    \caption*{SwinIR}
       \includegraphics[width=.98\textwidth]{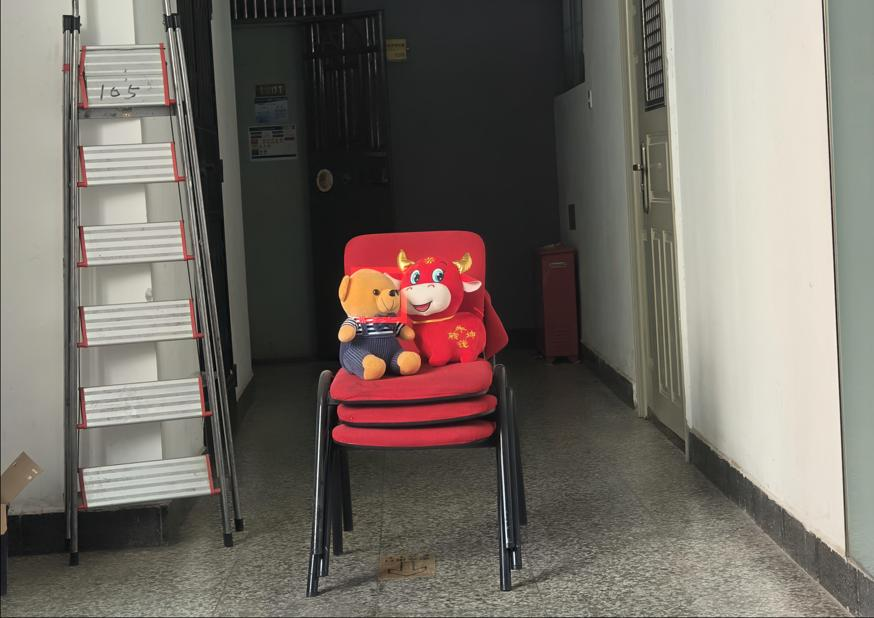}
       \includegraphics[width=.98\textwidth]{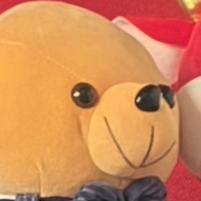}
       \includegraphics[width=.98\textwidth]{./compare/gt/771_crop.jpg}
        % \vspace{-6pt}
        \caption*{GT}
    \end{minipage}
    \vspace{-10pt}
    \caption{Example results of different algorithms trained on CameraFusion vs. ReWiTe. Top: The full-image results of different algorithms trained on ReWiTe. Middle: Results focused on the red-box region, derived from algorithms trained on CameraFusion. Bottom: Results focused on the red-box region, derived from algorithms trained on ReWiTe. Since the difficulty of perceiving differences of full-image results in compressed image size, only one full-image result is shown in the top line.
    }
    \label{fig: result compare10}
\end{figure*}

\begin{figure*}
    \centering
    \begin{minipage}[b]{0.138\textwidth}
        \centering
        \setlength{\abovecaptionskip}{0.005cm}
       % \includegraphics[width=.98\textwidth]{./compare/dcsr/615.jpg}
       % \includegraphics[width=.98\textwidth]{./compare/dcsr/615_crop.jpg}
       % \includegraphics[width=.98\textwidth]{./compare/dcsr-fin/615_crop.jpg}
    %    \includegraphics[width=.98\textwidth]{./compare/gt/615_crop.jpg}
    %    \caption*{srntt}
       \includegraphics[width=.98\textwidth]{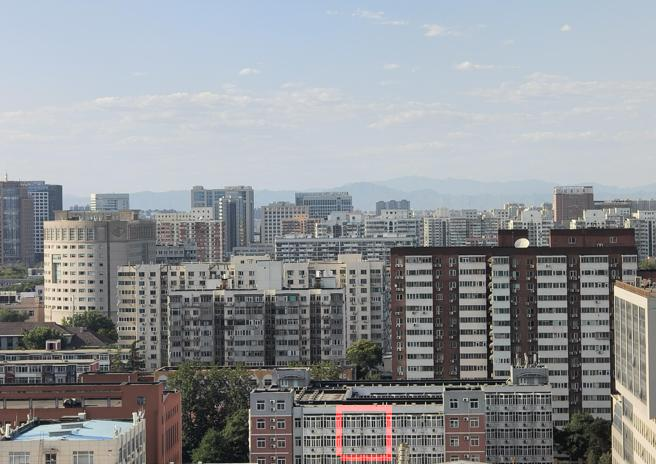}
       \includegraphics[width=.98\textwidth]{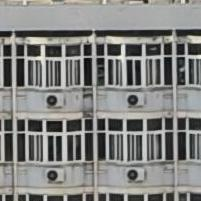}
       \includegraphics[width=.98\textwidth]{./compare/tele/809_crop.jpg}
       % \includegraphics[width=.98\textwidth]{./compare/tele/809_crop.jpg}
    %    \includegraphics[width=.98\textwidth]{./compare/gt/809_crop.jpg}
        % \vspace{-6pt}
        \caption*{\bf{Input T}}
    \end{minipage}
    \begin{minipage}[b]{0.138\textwidth}
    \centering
        \setlength{\abovecaptionskip}{0.005cm}
       % \includegraphics[width=.98\textwidth]{./compare/dcsr/615.jpg}
       % \includegraphics[width=.98\textwidth]{./compare/dcsr/615_crop.jpg}
       % \includegraphics[width=.98\textwidth]{./compare/dcsr-fin/615_crop.jpg}
    %    \includegraphics[width=.98\textwidth]{./compare/gt/615_crop.jpg}
    %    \caption*{srntt}
       \includegraphics[width=.98\textwidth]{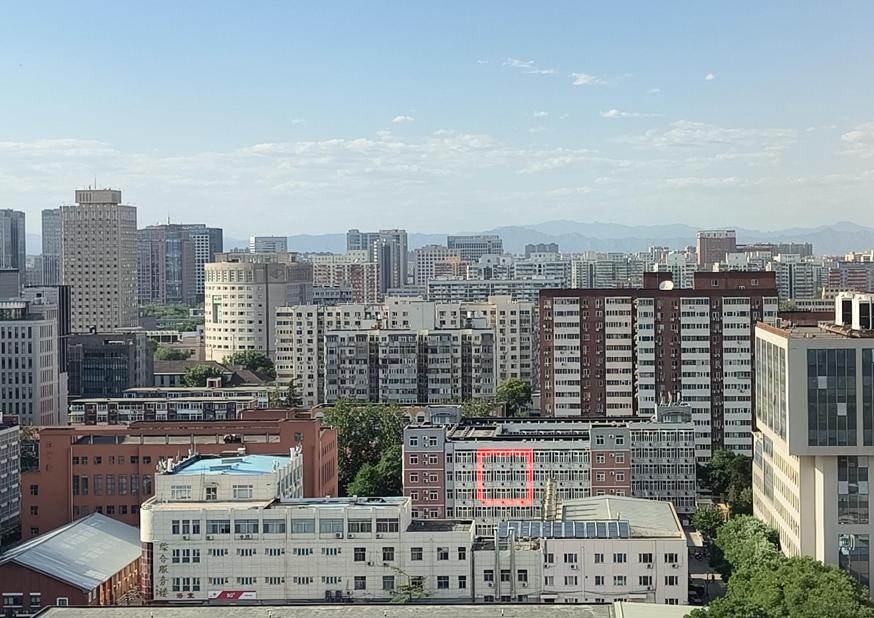}
       \includegraphics[width=.98\textwidth]{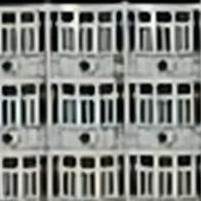}
       \includegraphics[width=.98\textwidth]{./compare/w+t/809_crop.jpg}
       % \includegraphics[width=.98\textwidth]{./compare/tele/809_crop.jpg}
    %    \includegraphics[width=.98\textwidth]{./compare/gt/809_crop.jpg}
        % \vspace{-6pt}
        \caption*{\bf{Input W}}
    \end{minipage}
    \begin{minipage}[b]{0.138\textwidth}
        \centering
        \setlength{\abovecaptionskip}{0.005cm}
       % \includegraphics[width=.98\textwidth]{./compare/dcsr/615.jpg}
       % \includegraphics[width=.98\textwidth]{./compare/dcsr/615_crop.jpg}
       % \includegraphics[width=.98\textwidth]{./compare/dcsr-fin/615_crop.jpg}
    %    \includegraphics[width=.98\textwidth]{./compare/gt/615_crop.jpg}
    %    \caption*{srntt}
       \includegraphics[width=.98\textwidth]{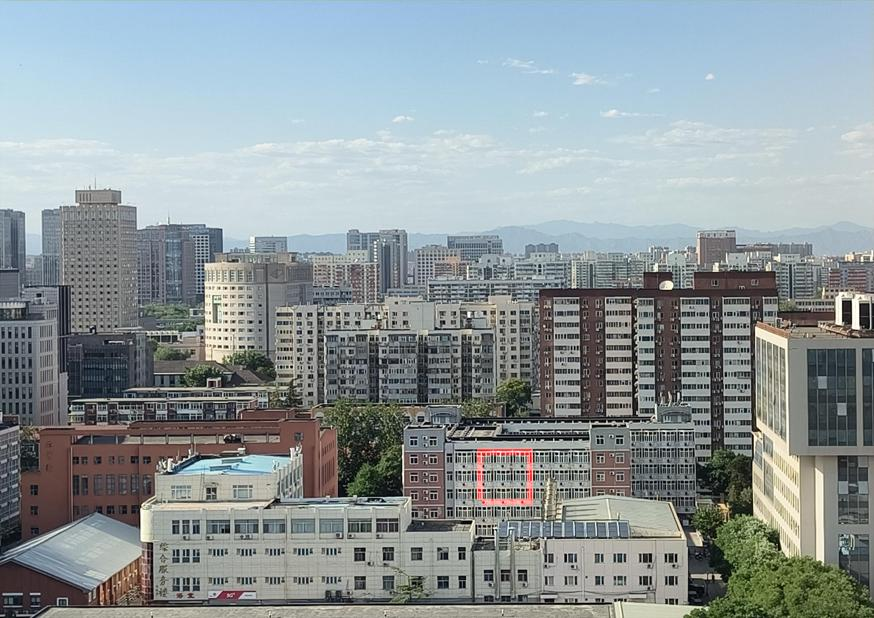}
       \includegraphics[width=.98\textwidth]{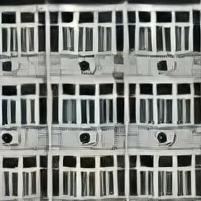}
       \includegraphics[width=.98\textwidth]{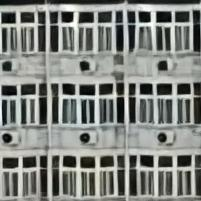}
    %    \includegraphics[width=.98\textwidth]{./compare/gt/809_crop.jpg}
        % \vspace{-6pt}
        \caption*{C2-matching}
    \end{minipage}
    \begin{minipage}[b]{0.138\textwidth}
        \centering
        \setlength{\abovecaptionskip}{0.005cm}
       % \includegraphics[width=.98\textwidth]{./compare/dcsr/615.jpg}
       % \includegraphics[width=.98\textwidth]{./compare/dcsr/615_crop.jpg}
       % \includegraphics[width=.98\textwidth]{./compare/dcsr-fin/615_crop.jpg}
    %    \includegraphics[width=.98\textwidth]{./compare/gt/615_crop.jpg}
    %    \caption*{srntt}
       \includegraphics[width=.98\textwidth]{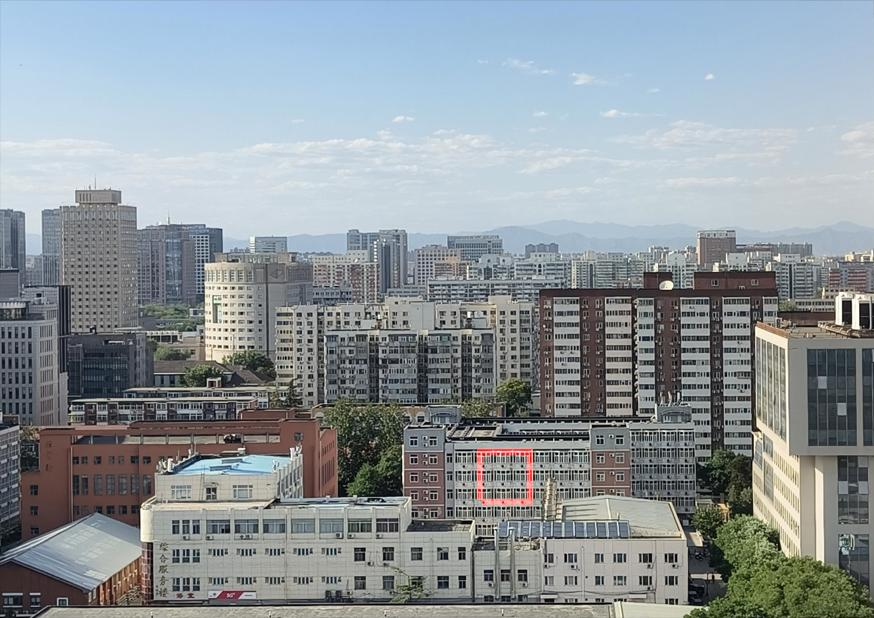}
       \includegraphics[width=.98\textwidth]{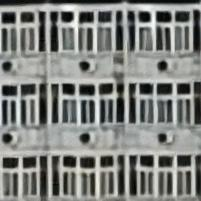}
       \includegraphics[width=.98\textwidth]{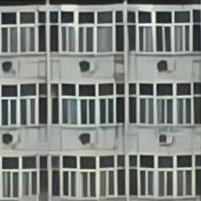}
    %    \includegraphics[width=.98\textwidth]{./compare/gt/809_crop.jpg}
        % \vspace{-6pt}
        \caption*{DCSR}
    \end{minipage}
    \begin{minipage}[b]{0.138\textwidth}
        \centering
        \setlength{\abovecaptionskip}{0.005cm}
       % \includegraphics[width=.98\textwidth]{./compare/selfdzsr/615.jpg}
       % \includegraphics[width=.98\textwidth]{./compare/selfdzsr/615_crop.jpg}
       % \includegraphics[width=.98\textwidth]{./compare/selfdzsr-fin/615_crop.jpg}
    %    \includegraphics[width=.98\textwidth]{./compare/gt/615_crop.jpg}
    %    \caption*{srntt}
       \includegraphics[width=.98\textwidth]{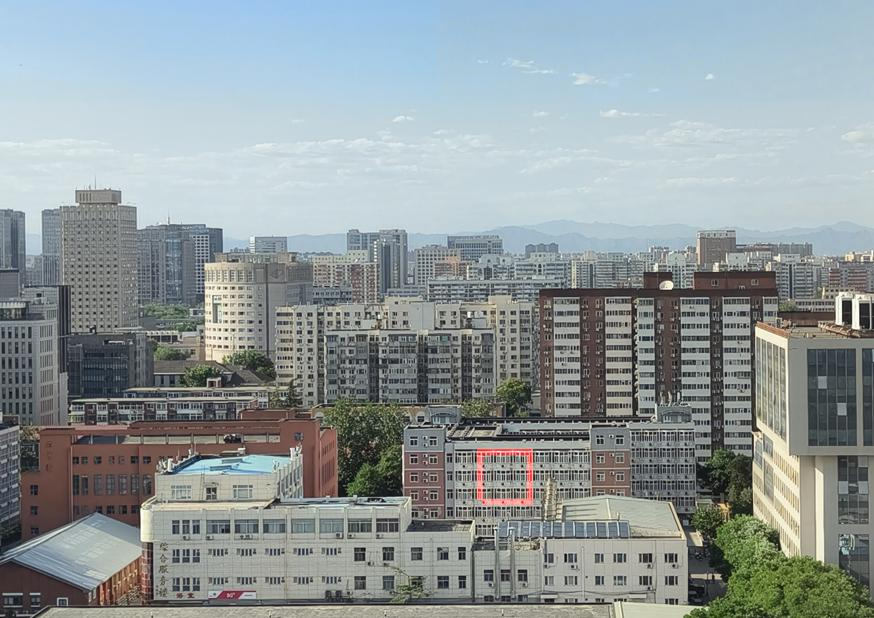}
       \includegraphics[width=.98\textwidth]{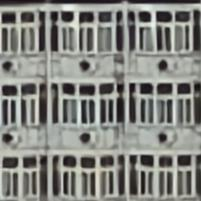}
       \includegraphics[width=.98\textwidth]{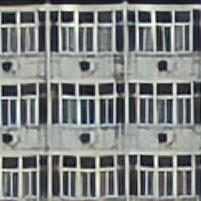}
    %    \includegraphics[width=.98\textwidth]{./compare/gt/809_crop.jpg}
        % \vspace{-6pt}
        \caption*{SelfDZSR}
    \end{minipage}
    \begin{minipage}[b]{0.138\textwidth}
        \centering
        \setlength{\abovecaptionskip}{0.005cm}
       % \includegraphics[width=.98\textwidth]{./compare/zedusr/615.jpg}
       % \includegraphics[width=.98\textwidth]{./compare/zedusr/615_crop.jpg}
       % \includegraphics[width=.98\textwidth]{./compare/zedusr-fin/615_crop.jpg}
    %    \includegraphics[width=.98\textwidth]{./compare/gt/615_crop.jpg}
    %    \caption*{srntt}
       \includegraphics[width=.98\textwidth]{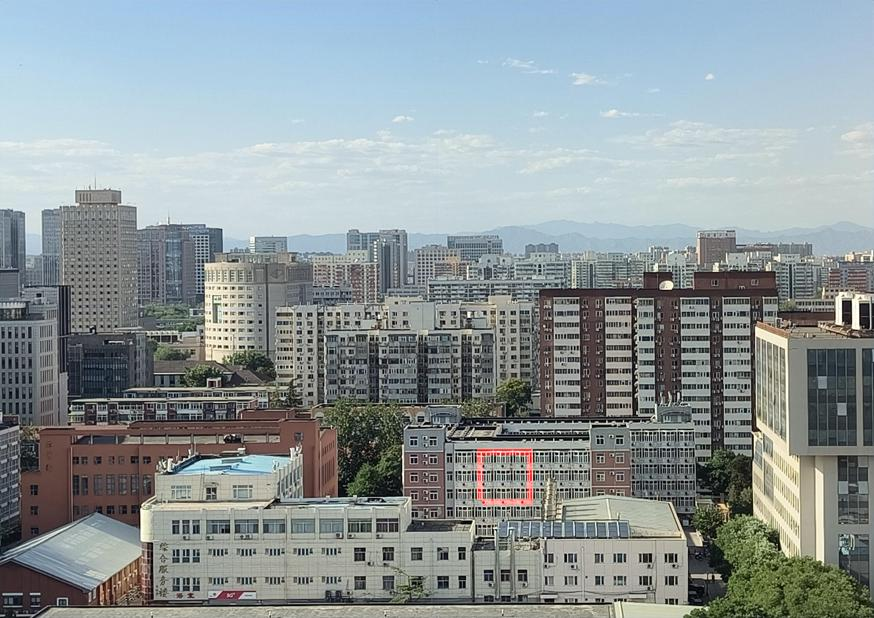}
       \includegraphics[width=.98\textwidth]{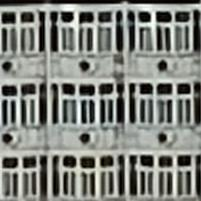}
       \includegraphics[width=.98\textwidth]{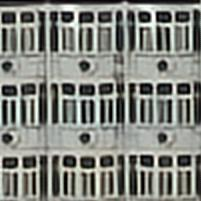}
    %    \includegraphics[width=.98\textwidth]{./compare/gt/809_crop.jpg}
        % \vspace{-6pt}
        \caption*{ZeDUSR}
    \end{minipage}
    \begin{minipage}[b]{0.138\textwidth}
        \centering
        \setlength{\abovecaptionskip}{0.005cm}
       % \includegraphics[width=.98\textwidth]{./compare/MASA/615.jpg}
       % \includegraphics[width=.98\textwidth]{./compare/MASA/615_crop.jpg}
       % \includegraphics[width=.98\textwidth]{./compare/MASA-fin/615_crop.jpg}
    %    \includegraphics[width=.98\textwidth]{./compare/gt/615_crop.jpg}
    %    \caption*{srntt}
       \includegraphics[width=.98\textwidth]{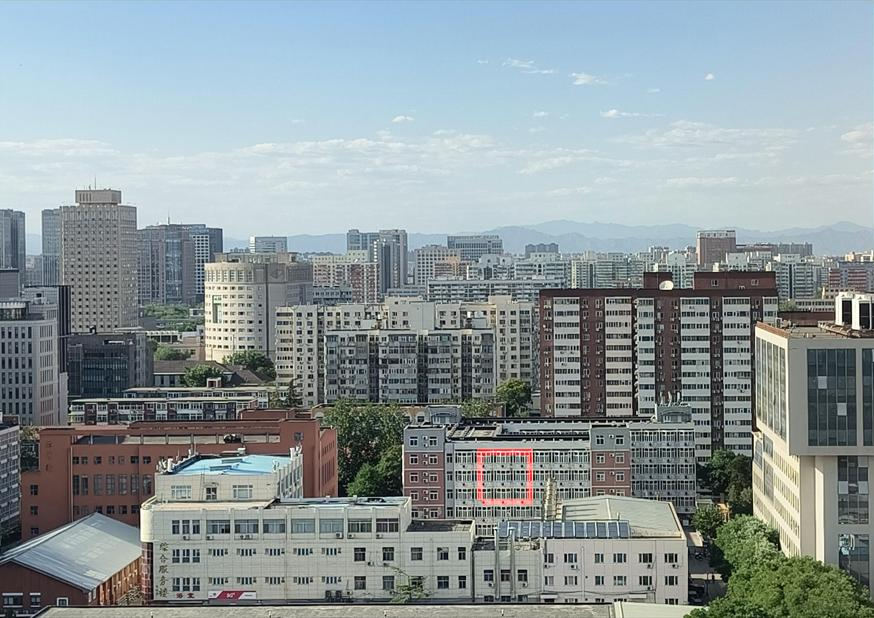}
       \includegraphics[width=.98\textwidth]{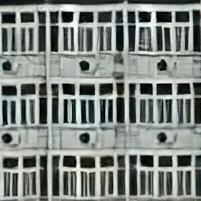}
       \includegraphics[width=.98\textwidth]{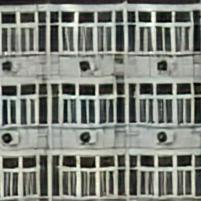}
    %    \includegraphics[width=.98\textwidth]{./compare/gt/809_crop.jpg}
        % \vspace{-6pt}
        \caption*{MASA}
    \end{minipage}
    \begin{minipage}[b]{0.138\textwidth}
        \centering
        \setlength{\abovecaptionskip}{0.005cm}
       % \includegraphics[width=.98\textwidth]{./compare/ttsr/615.jpg}
       % \includegraphics[width=.98\textwidth]{./compare/ttsr/615_crop.jpg}
       % \includegraphics[width=.98\textwidth]{./compare/ttsr-fin/615_crop.jpg}
    %    \includegraphics[width=.98\textwidth]{./compare/gt/615_crop.jpg}
    %    \caption*{srntt}
       \includegraphics[width=.98\textwidth]{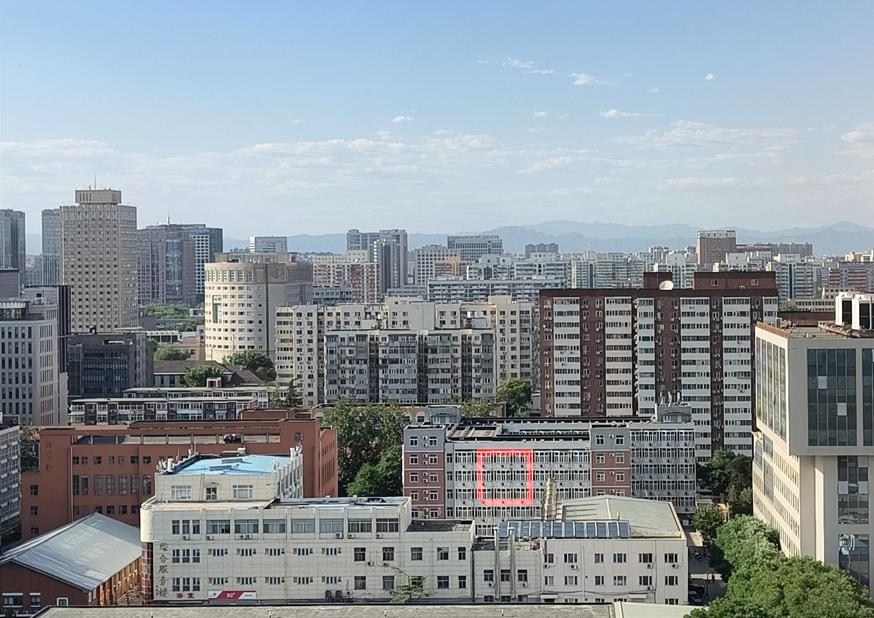}
       \includegraphics[width=.98\textwidth]{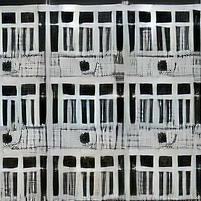}
       \includegraphics[width=.98\textwidth]{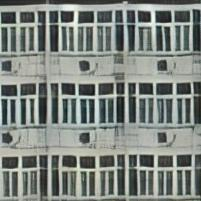}
    %    \includegraphics[width=.98\textwidth]{./compare/gt/809_crop.jpg}
        % \vspace{-6pt}
        \caption*{TTSR}
    \end{minipage}
    \begin{minipage}[b]{0.138\textwidth}
        \centering
        \setlength{\abovecaptionskip}{0.005cm}
       % \includegraphics[width=.98\textwidth]{./compare/srntt/615.jpg}
       % \includegraphics[width=.98\textwidth]{./compare/srntt/615_crop.jpg}
       % \includegraphics[width=.98\textwidth]{./compare/srntt-fin/615_crop.jpg}
    %    \includegraphics[width=.98\textwidth]{./compare/gt/615_crop.jpg}
    %    \caption*{srntt}
       \includegraphics[width=.98\textwidth]{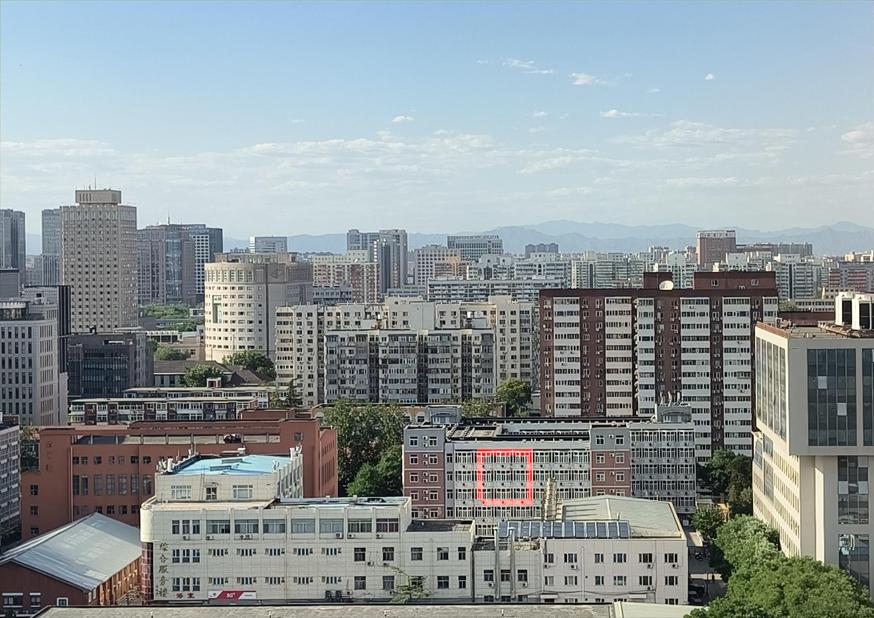}
       \includegraphics[width=.98\textwidth]{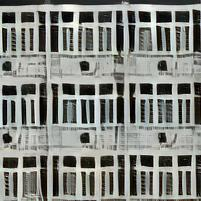}
       \includegraphics[width=.98\textwidth]{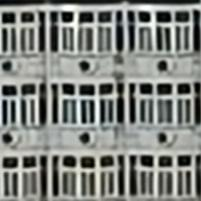}
    %    \includegraphics[width=.98\textwidth]{./compare/gt/809_crop.jpg}
        % \vspace{-6pt}
        \caption*{SRNTT}
    \end{minipage}
    \begin{minipage}[b]{0.138\textwidth}
        \centering
        \setlength{\abovecaptionskip}{0.005cm}
       % \includegraphics[width=.98\textwidth]{./compare/RCAN/615.jpg}
       % \includegraphics[width=.98\textwidth]{./compare/RCAN/615_crop.jpg}
       % \includegraphics[width=.98\textwidth]{./compare/RCAN-fin/615_crop.jpg}
    %    \includegraphics[width=.98\textwidth]{./compare/gt/615_crop.jpg}
    %    \caption*{RCAN}
       \includegraphics[width=.98\textwidth]{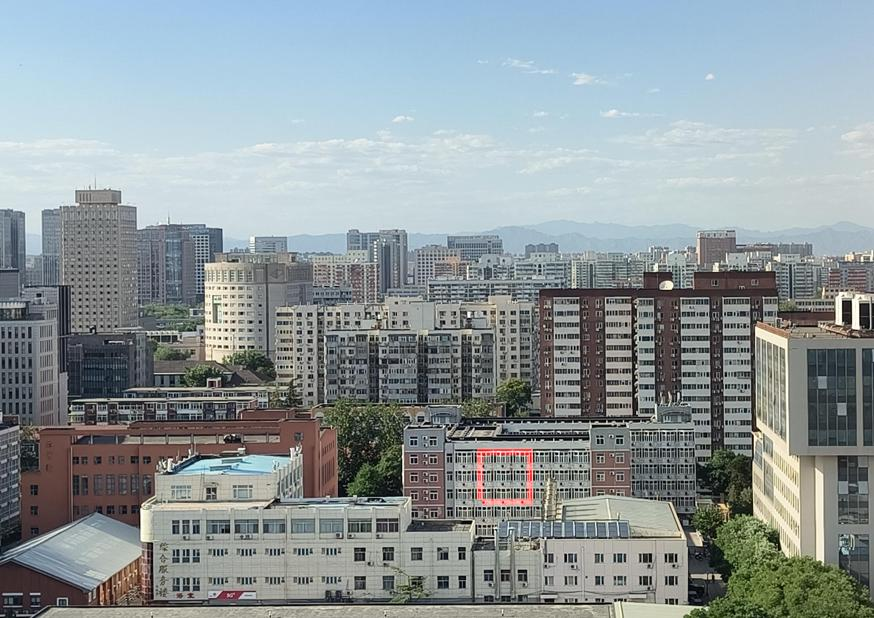}
       \includegraphics[width=.98\textwidth]{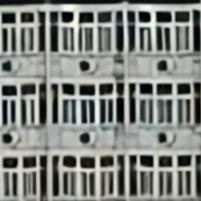}
       \includegraphics[width=.98\textwidth]{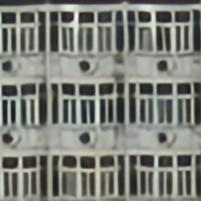}
    %    \includegraphics[width=.98\textwidth]{./compare/gt/809_crop.jpg}
        % \vspace{-6pt}
        \caption*{RCAN}
    \end{minipage}
    \begin{minipage}[b]{0.138\textwidth}
        \centering
        \setlength{\abovecaptionskip}{0.005cm}
       % \includegraphics[width=.98\textwidth]{./compare/EDSR/615.jpg}
       % \includegraphics[width=.98\textwidth]{./compare/EDSR/615_crop.jpg}
       % \includegraphics[width=.98\textwidth]{./compare/EDSR-fin/615_crop.jpg}
    %    \includegraphics[width=.98\textwidth]{./compare/gt/615_crop.jpg}
    %    \caption*{EDSR}
       \includegraphics[width=.98\textwidth]{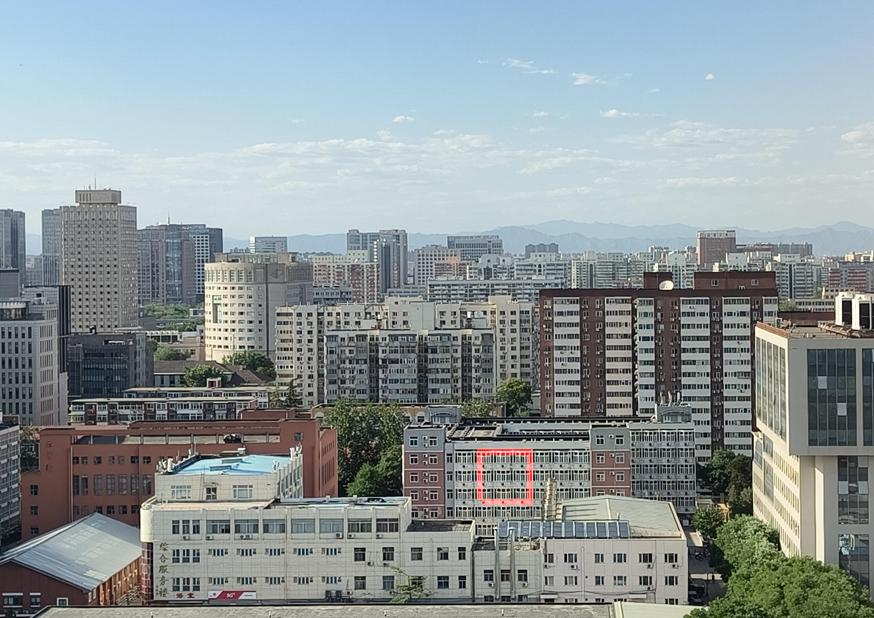}
       \includegraphics[width=.98\textwidth]{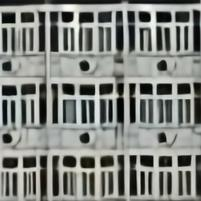}
       \includegraphics[width=.98\textwidth]{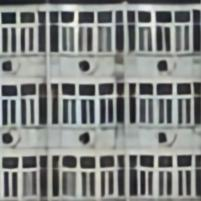}
    %    \includegraphics[width=.98\textwidth]{./compare/gt/809_crop.jpg}
        % \vspace{-6pt}
        \caption*{EDSR}
    \end{minipage}
    \begin{minipage}[b]{0.138\textwidth}
        \centering
        \setlength{\abovecaptionskip}{0.005cm}
       % \includegraphics[width=.98\textwidth]{./compare/Real_ESRGAN/615.jpg}
       % \includegraphics[width=.98\textwidth]{./compare/Real_ESRGAN/615_crop.jpg}
       % \includegraphics[width=.98\textwidth]{./compare/Real_ESRGAN-fin/615_crop.jpg}
    %    \includegraphics[width=.98\textwidth]{./compare/gt/615_crop.jpg}
    %    \caption*{Real_ESRGAN}
       \includegraphics[width=.98\textwidth]{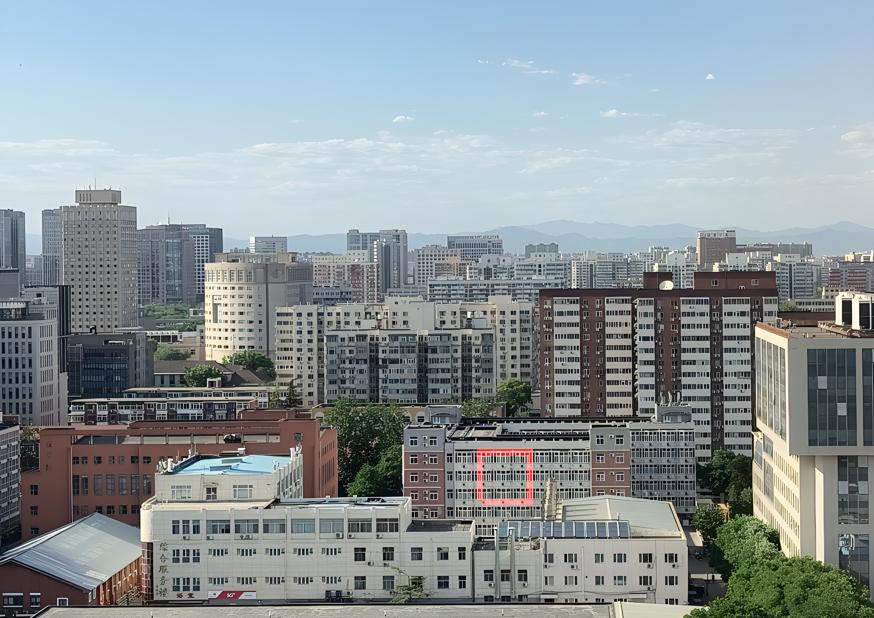}
       \includegraphics[width=.98\textwidth]{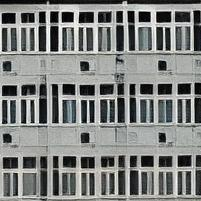}
       \includegraphics[width=.98\textwidth]{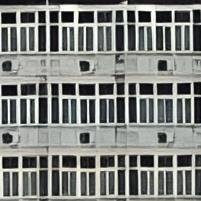}
    %    \includegraphics[width=.98\textwidth]{./compare/gt/809_crop.jpg}
        % \vspace{-6pt}
        \caption*{Real-ESRGAN}
    \end{minipage}
    \begin{minipage}[b]{0.138\textwidth}
        \centering
        \setlength{\abovecaptionskip}{0.005cm}
       % \includegraphics[width=.98\textwidth]{./compare/swinir/615.jpg}
       % \includegraphics[width=.98\textwidth]{./compare/swinir/615_crop.jpg}
       % \includegraphics[width=.98\textwidth]{./compare/swinir-fin/615_crop.jpg}
    %    \includegraphics[width=.98\textwidth]{./compare/gt/615_crop.jpg}
    %    \caption*{SwinIR}
       \includegraphics[width=.98\textwidth]{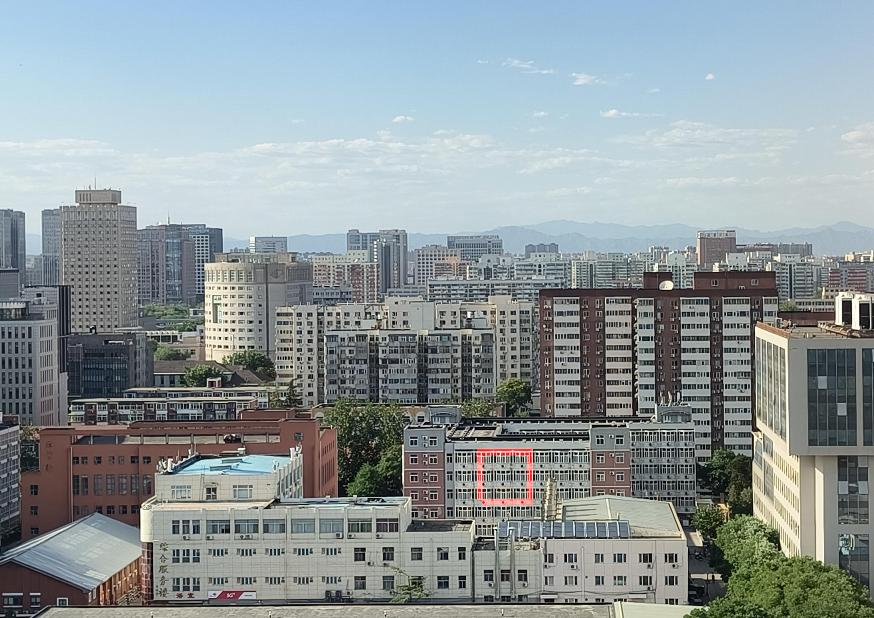}
       \includegraphics[width=.98\textwidth]{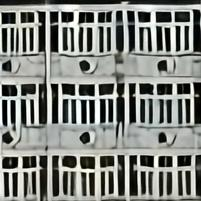}
       \includegraphics[width=.98\textwidth]{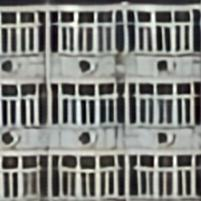}
    %    \includegraphics[width=.98\textwidth]{./compare/gt/809_crop.jpg}
        % \vspace{-6pt}
        \caption*{SwinIR}
    \end{minipage}
    \begin{minipage}[b]{0.138\textwidth}
        \centering
        \setlength{\abovecaptionskip}{0.005cm}
       % \includegraphics[width=.98\textwidth]{./compare/gt/615.jpg}
    %    \includegraphics[width=.98\textwidth]{./compare/swinir/615_crop.jpg}
    %    \includegraphics[width=.98\textwidth]{./compare/swinir-fin/615_crop.jpg}
       % \includegraphics[width=.98\textwidth]{./compare/gt/615_crop.jpg}
    %    \caption*{SwinIR}
       \includegraphics[width=.98\textwidth]{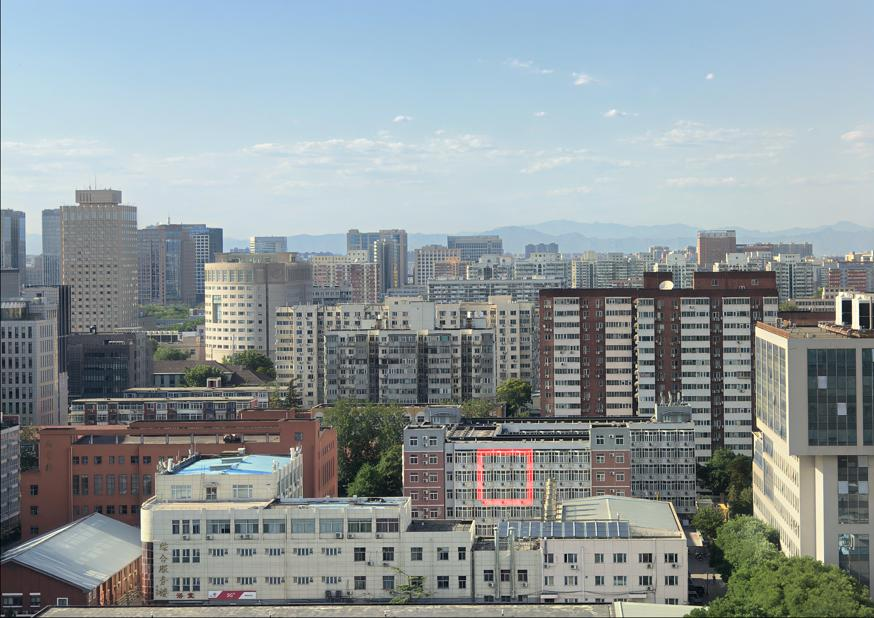}
       \includegraphics[width=.98\textwidth]{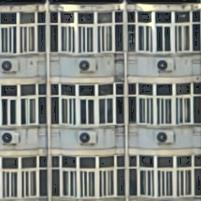}
       \includegraphics[width=.98\textwidth]{./compare/gt/809_crop.jpg}
        % \vspace{-6pt}
        \caption*{GT}
    \end{minipage}
    \vspace{-10pt}
    \caption{Example results of different algorithms trained on CameraFusion vs. ReWiTe. Top: The full-image results of different algorithms trained on ReWiTe. Middle: Results focused on the red-box region, derived from algorithms trained on CameraFusion. Bottom: Results focused on the red-box region, derived from algorithms trained on ReWiTe. Since the difficulty of perceiving differences of full-image results in compressed image size, only one full-image result is shown in the top line.
    }
    \label{fig: result compare11}
\end{figure*}
